# Supplementary material for: Self-learn to Explain Siamese Networks Robustly
Source: arXiv:2109.07371 source file (2021-09-15)
Supplement: Supplementary file 1 [file supp.tex]

\section*{Supplement}

\subsection{More details about sensitivity study}
\begin{figure}[t]
    \centering
\begin{minipage}{.15\textwidth}
    \includegraphics[width=\textwidth]{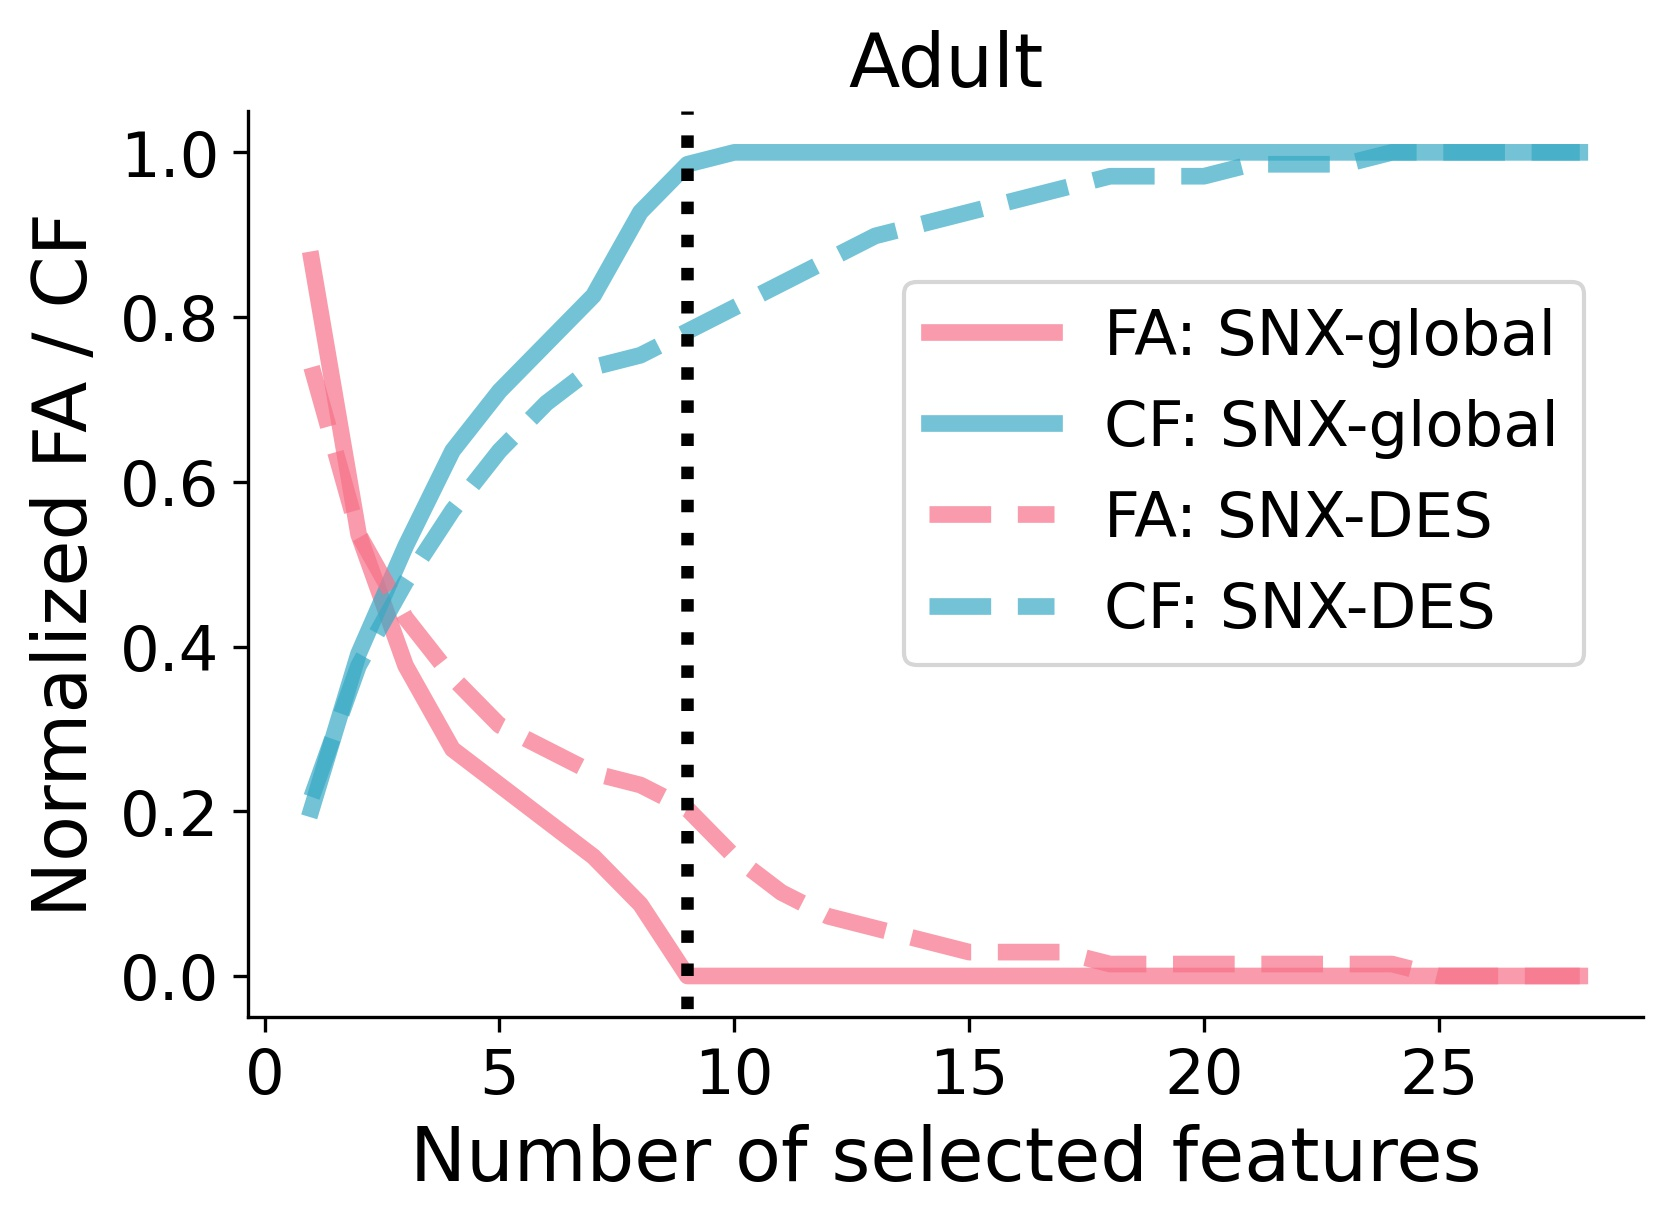}
\end{minipage}%
\begin{minipage}{.15\textwidth}
    \includegraphics[width=\textwidth]{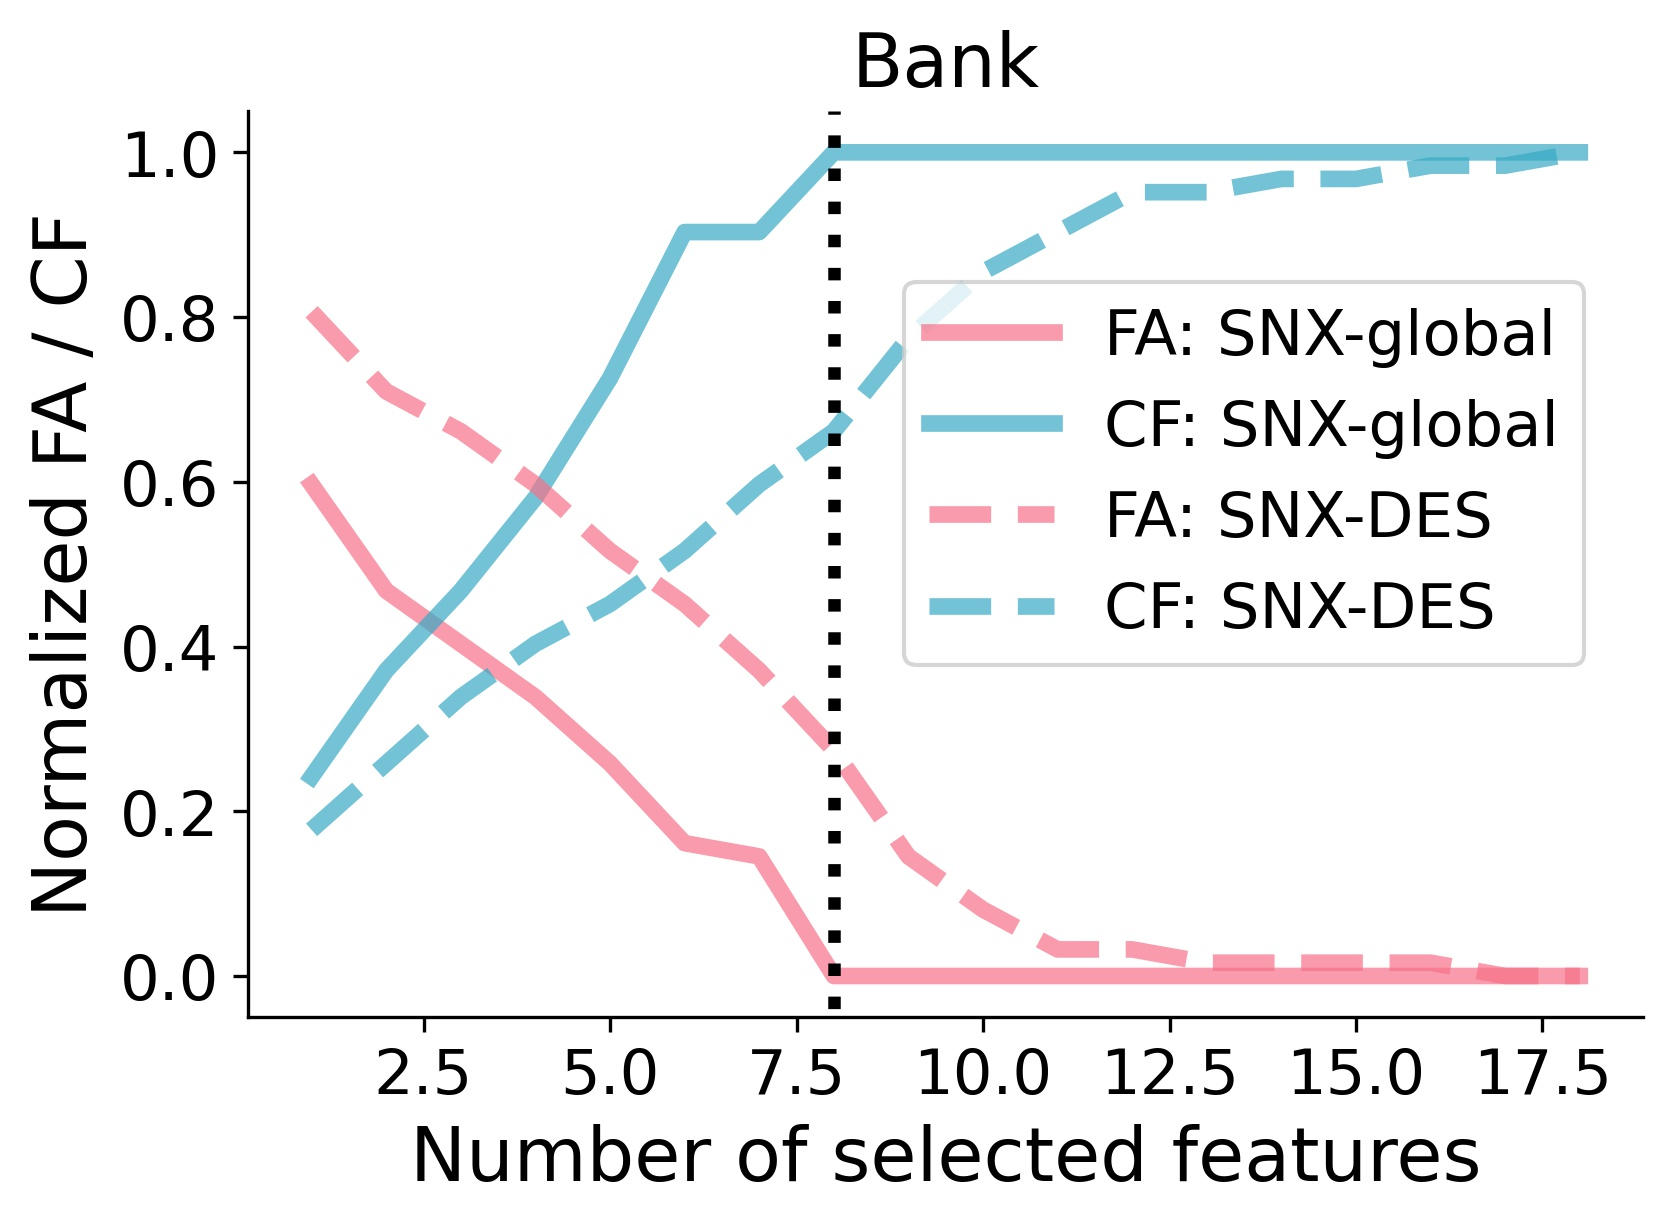}
\end{minipage}%
\begin{minipage}{.15\textwidth}
    \includegraphics[width=\textwidth]{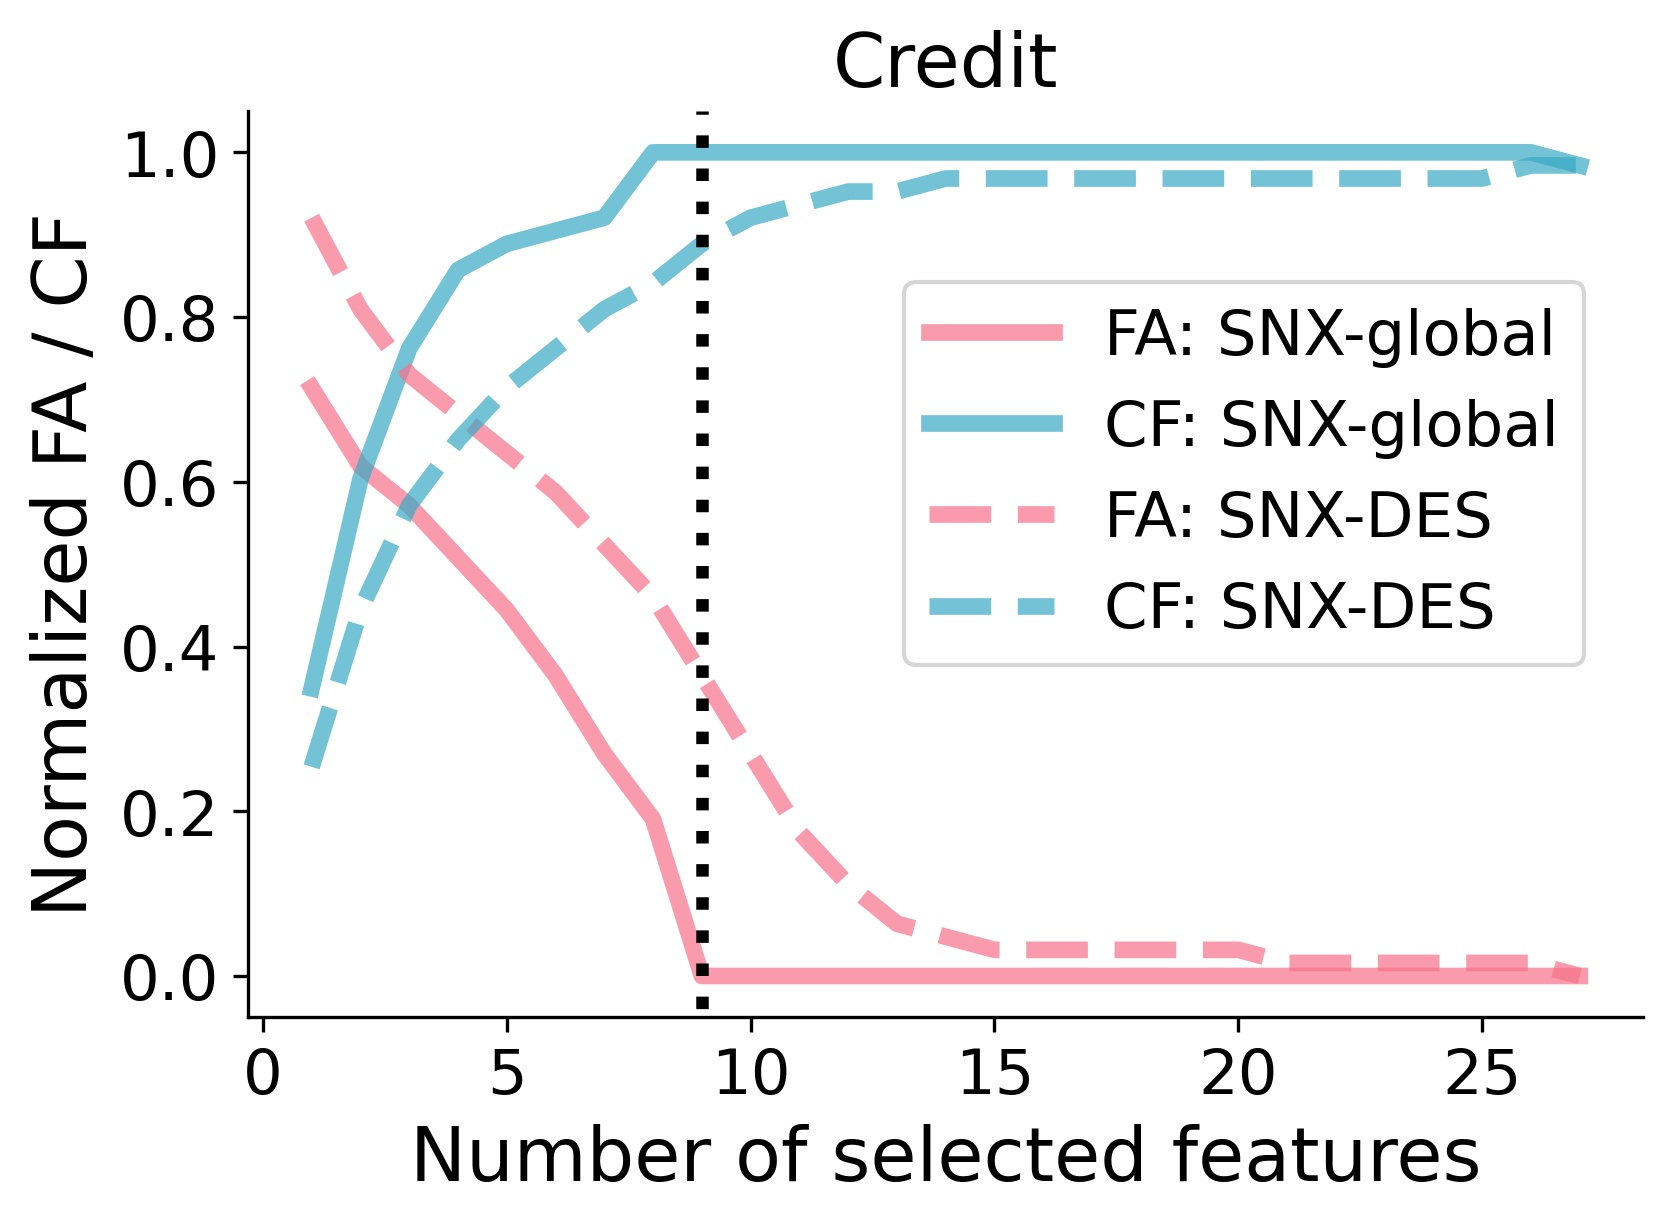}
\end{minipage}\\
\begin{minipage}{.15\textwidth}
    \includegraphics[width=\textwidth]{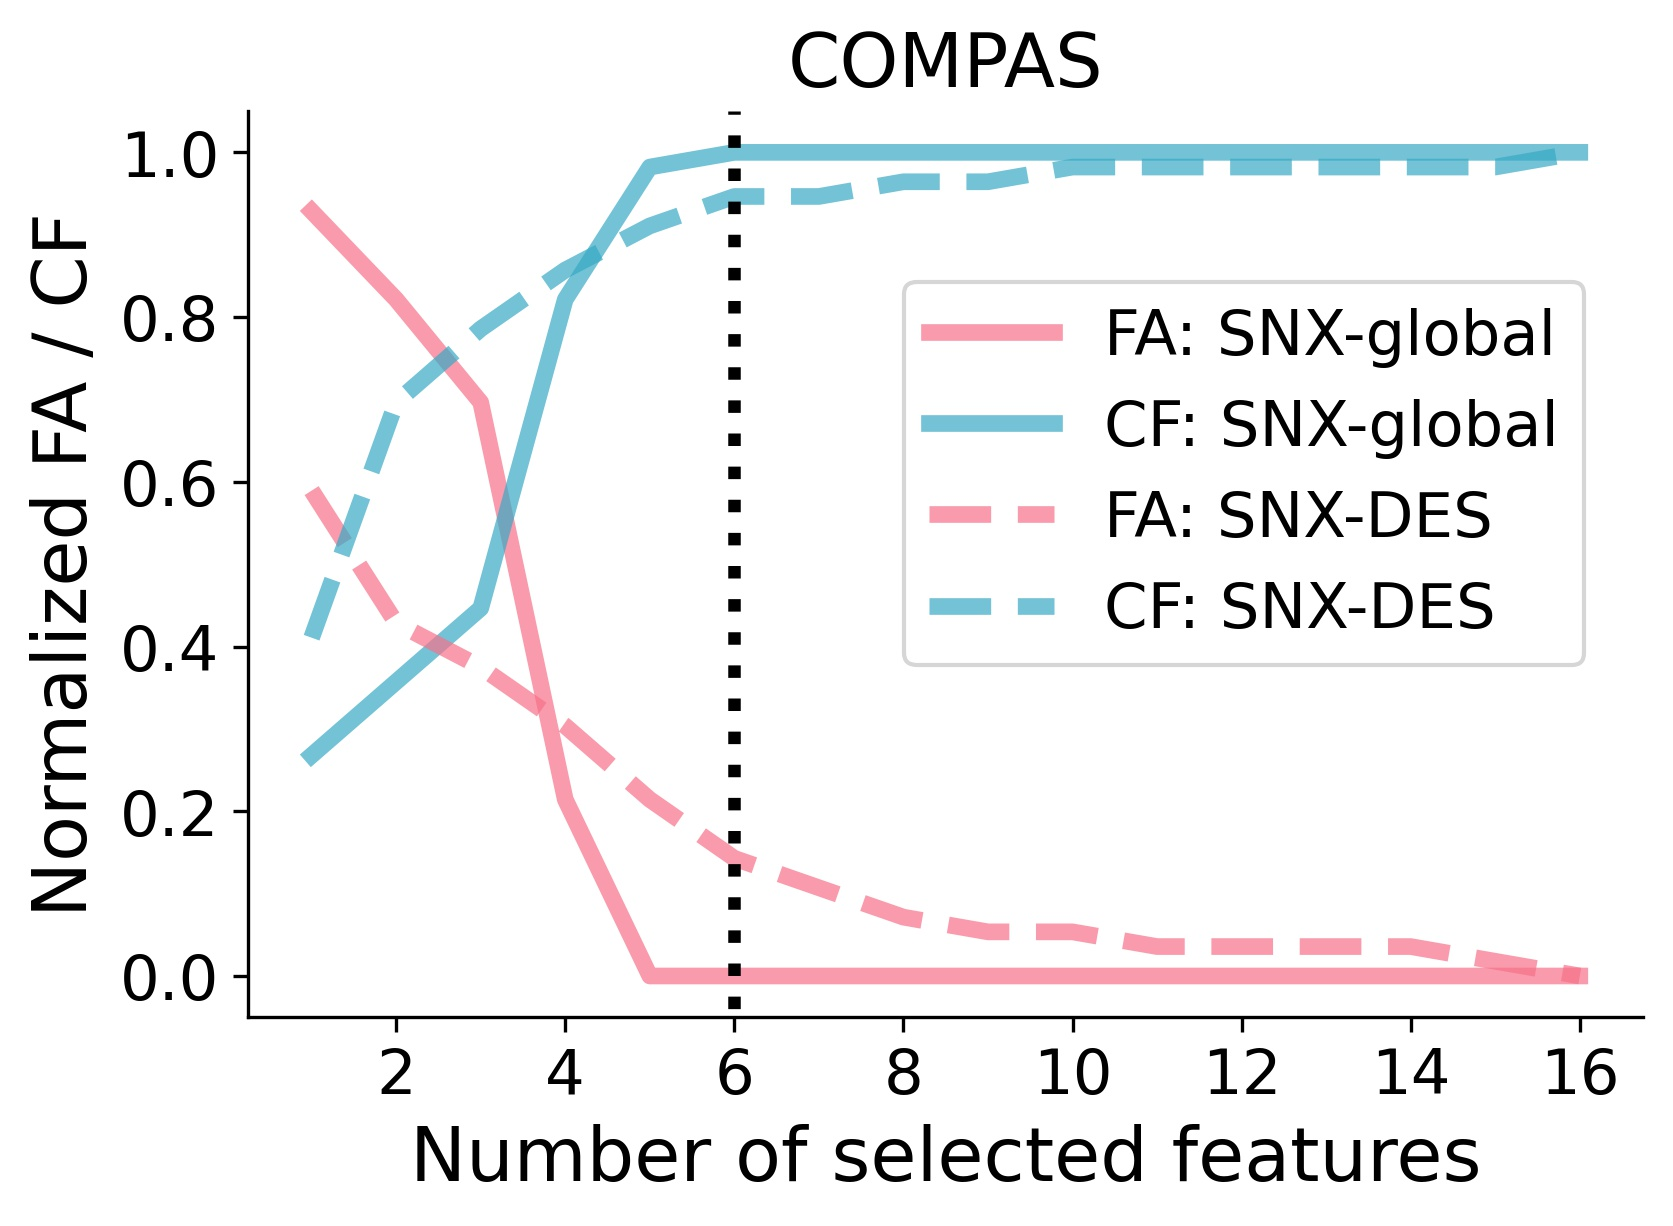}
\end{minipage}%
\begin{minipage}{.15\textwidth}
    \includegraphics[width=\textwidth]{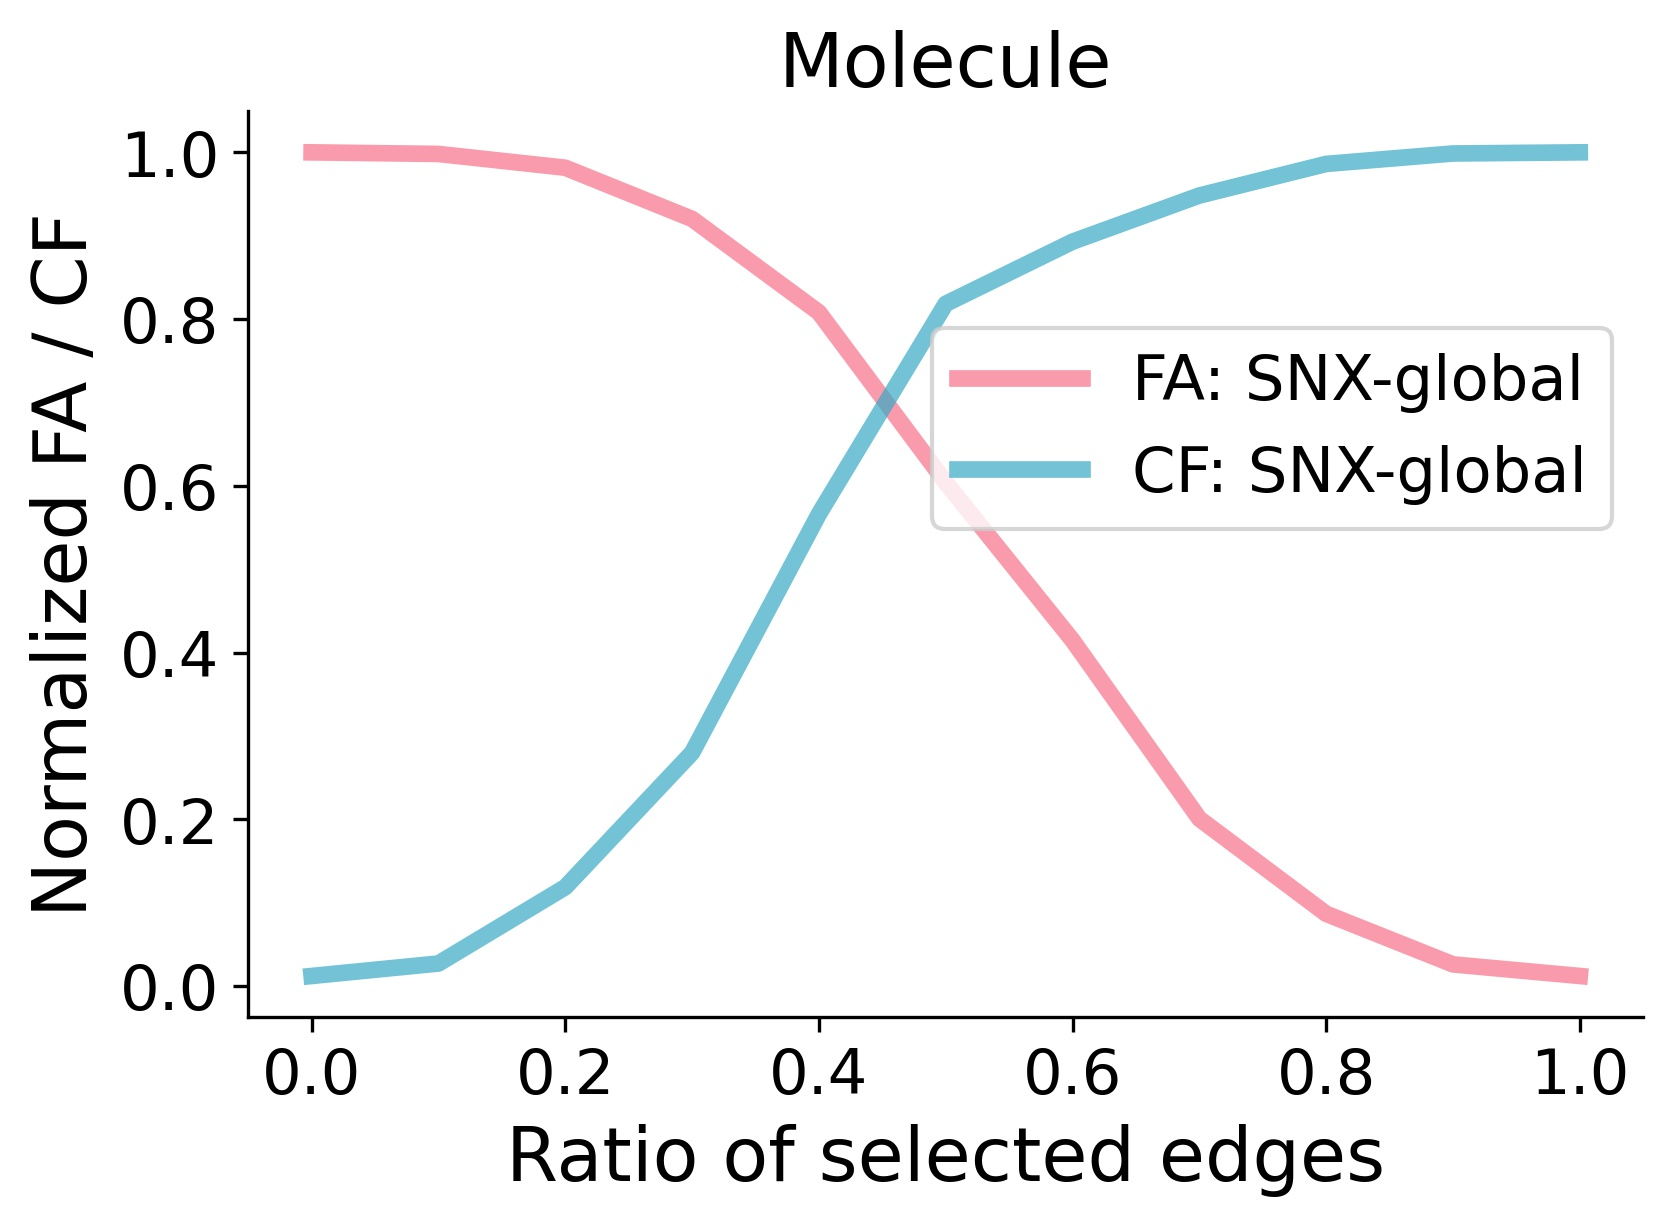}
\end{minipage}%
\begin{minipage}{.15\textwidth}
    \includegraphics[width=\textwidth]{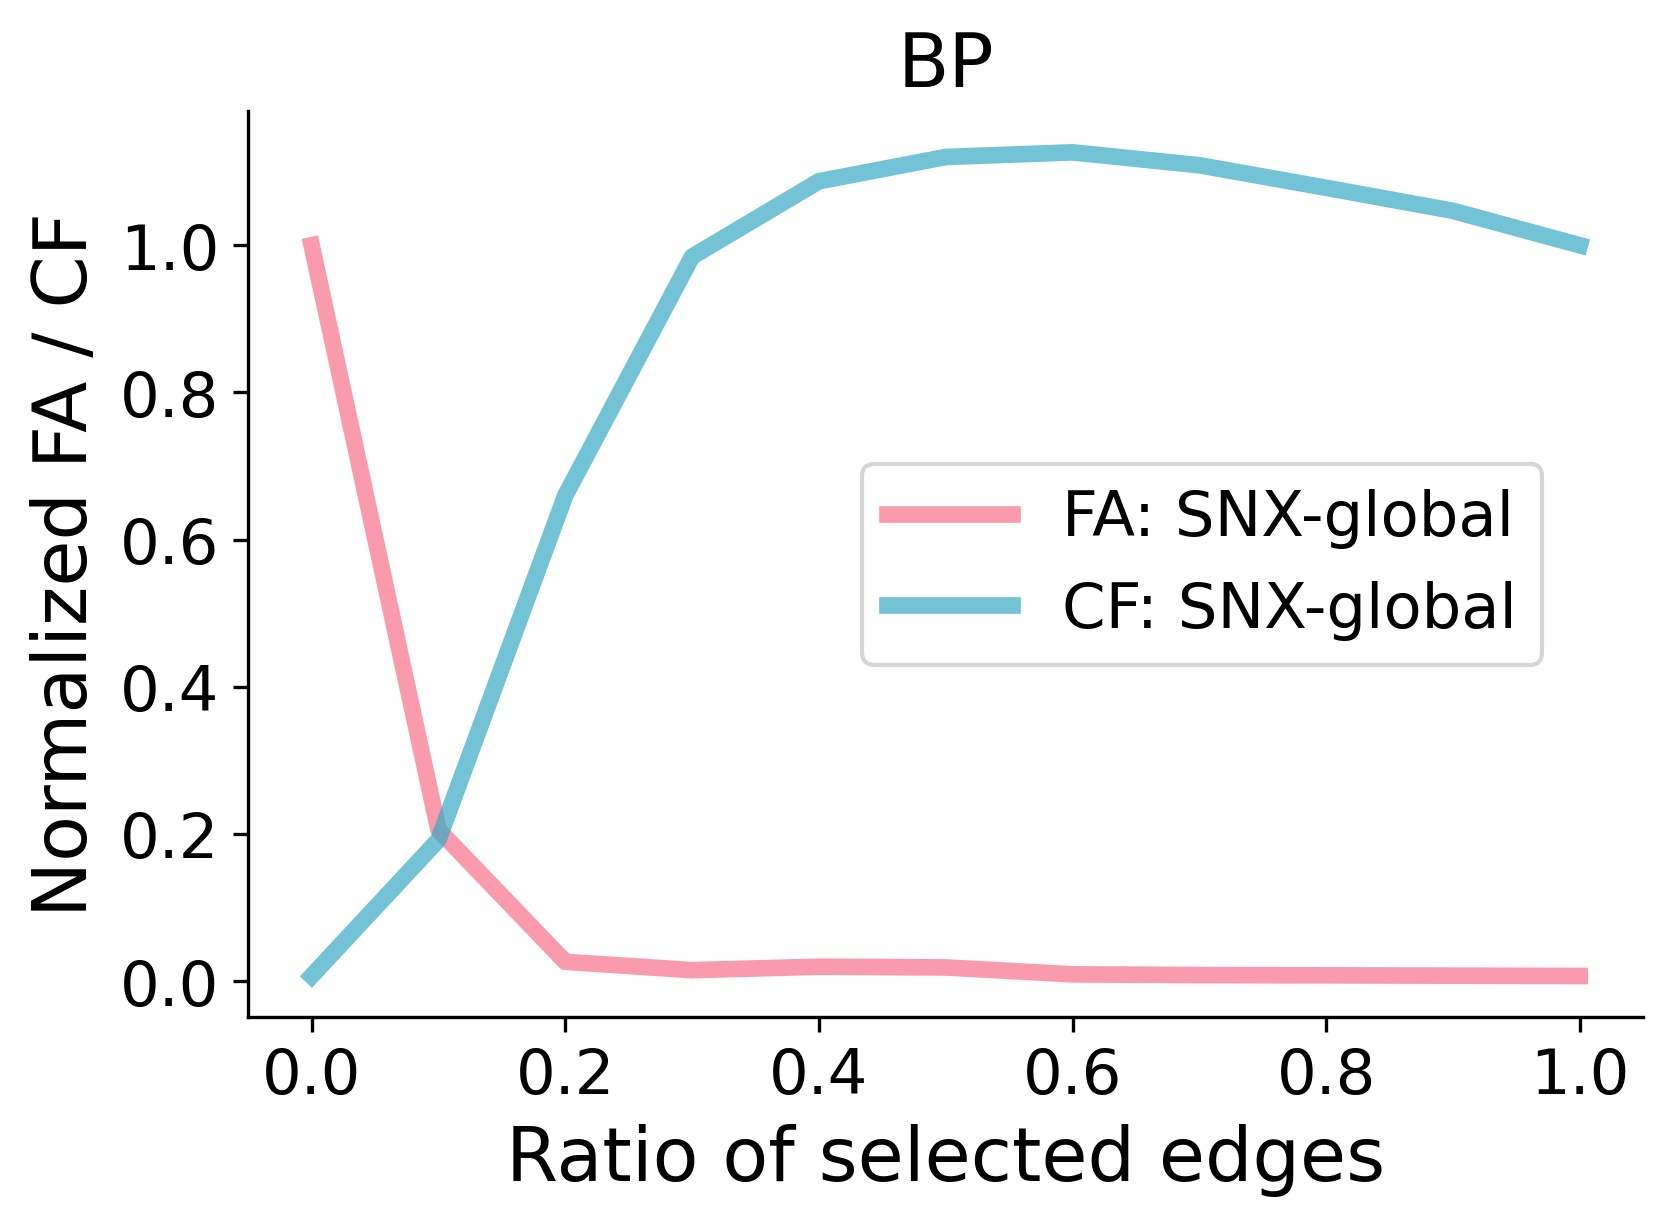}
\end{minipage}%
    \caption{\small The \textit{faithfulness} and \textit{counterfactual} of the global masks, 
    with respect to the number/percentage of the selected features (or edges).
    The vertical black dotted lines in tabular datasets indicate the number of major features.
    % \textcolor{blue}{Settings: It is a complete results of Figure 6 on all datasets.}
    }
    \label{fig:global_faithfulness}
\end{figure}

\begin{figure}[t]
    \centering
\begin{minipage}{.15\textwidth}
    \includegraphics[width=\textwidth]{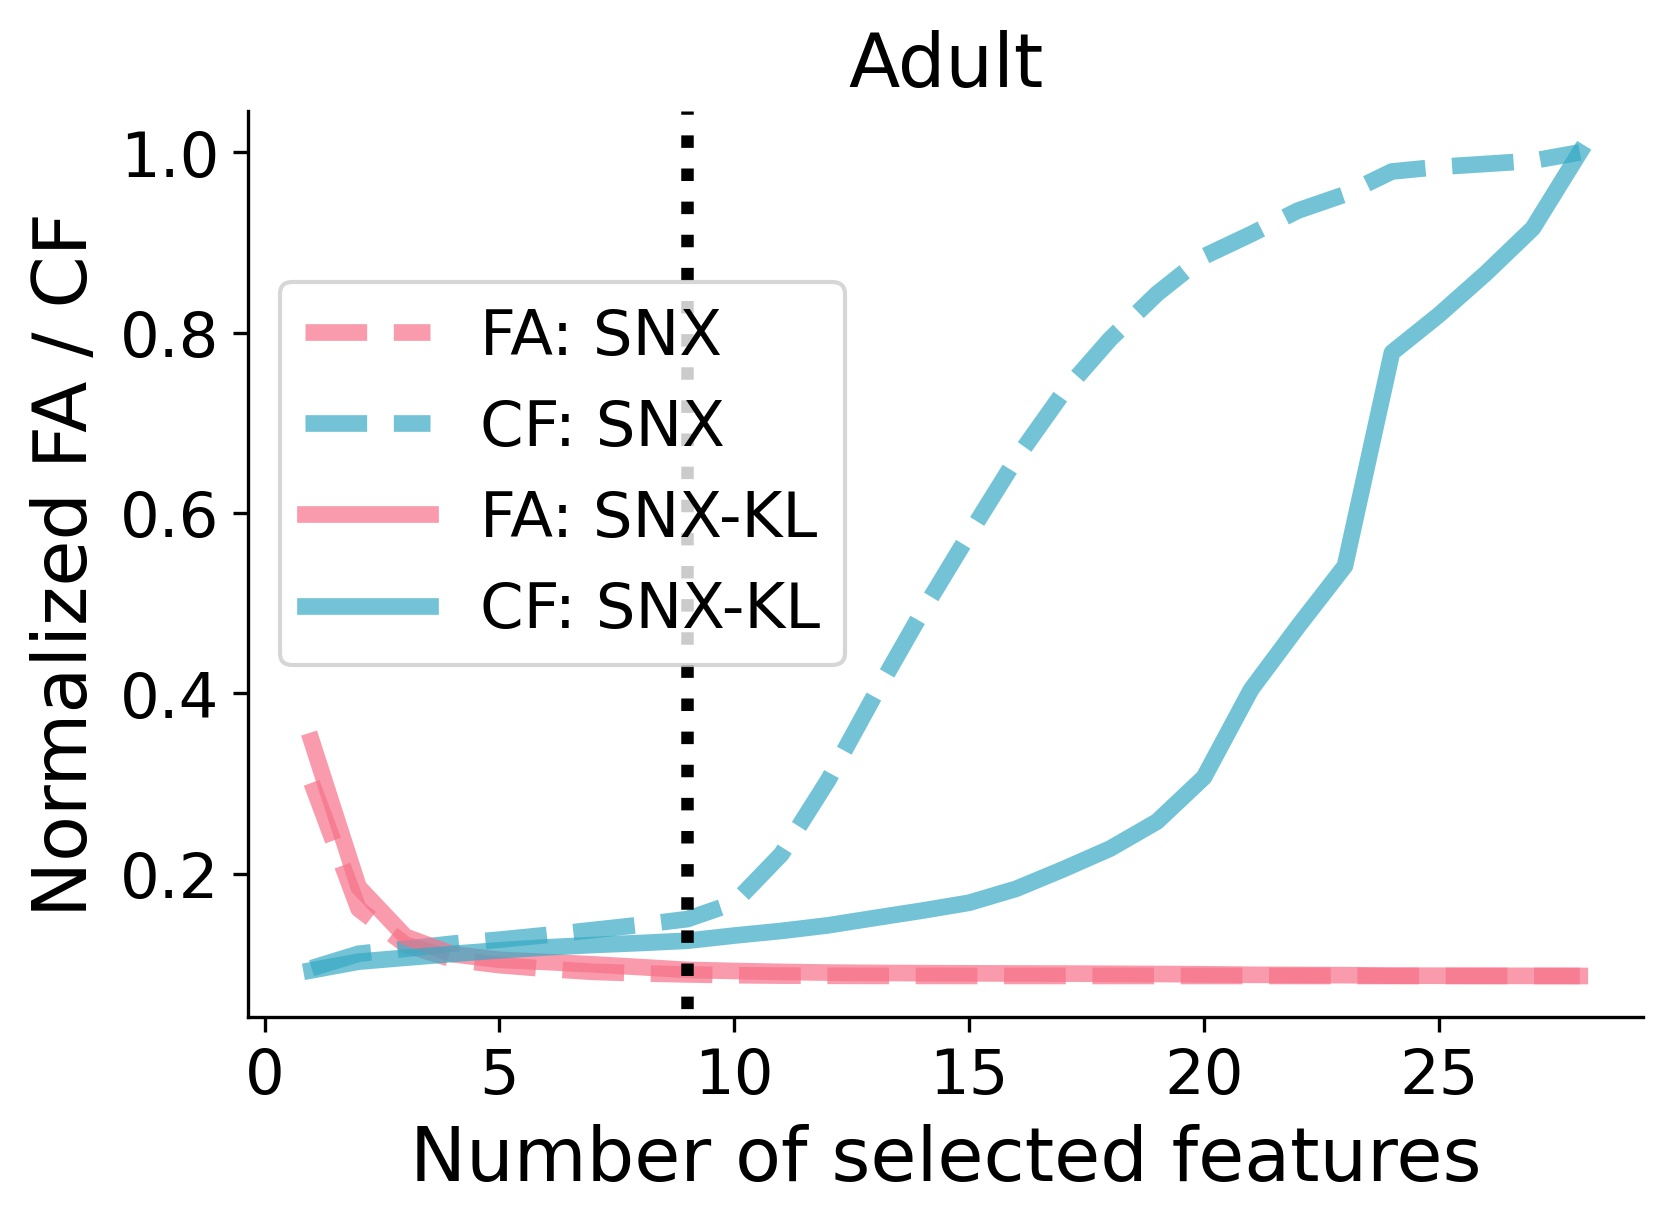}
\end{minipage}%
\begin{minipage}{.15\textwidth}
    \includegraphics[width=\textwidth]{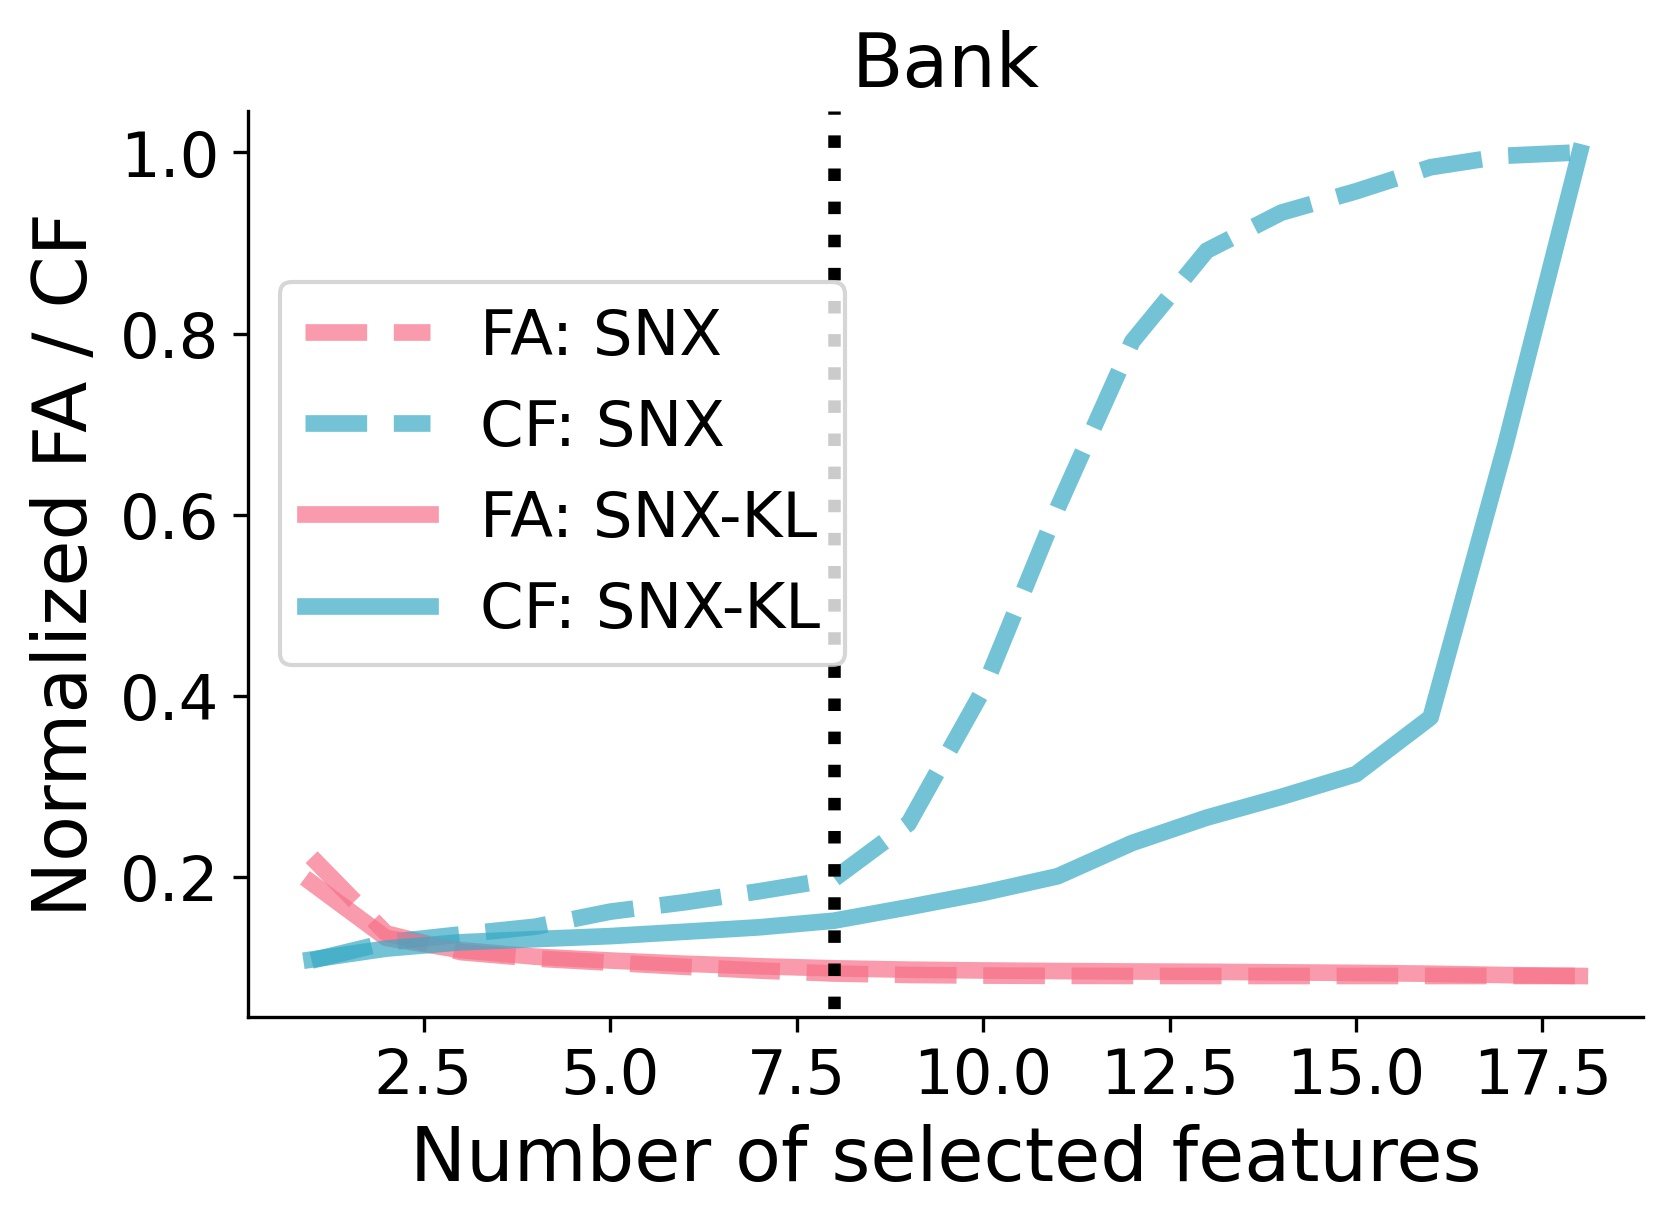}
\end{minipage}%
\begin{minipage}{.15\textwidth}
    \includegraphics[width=\textwidth]{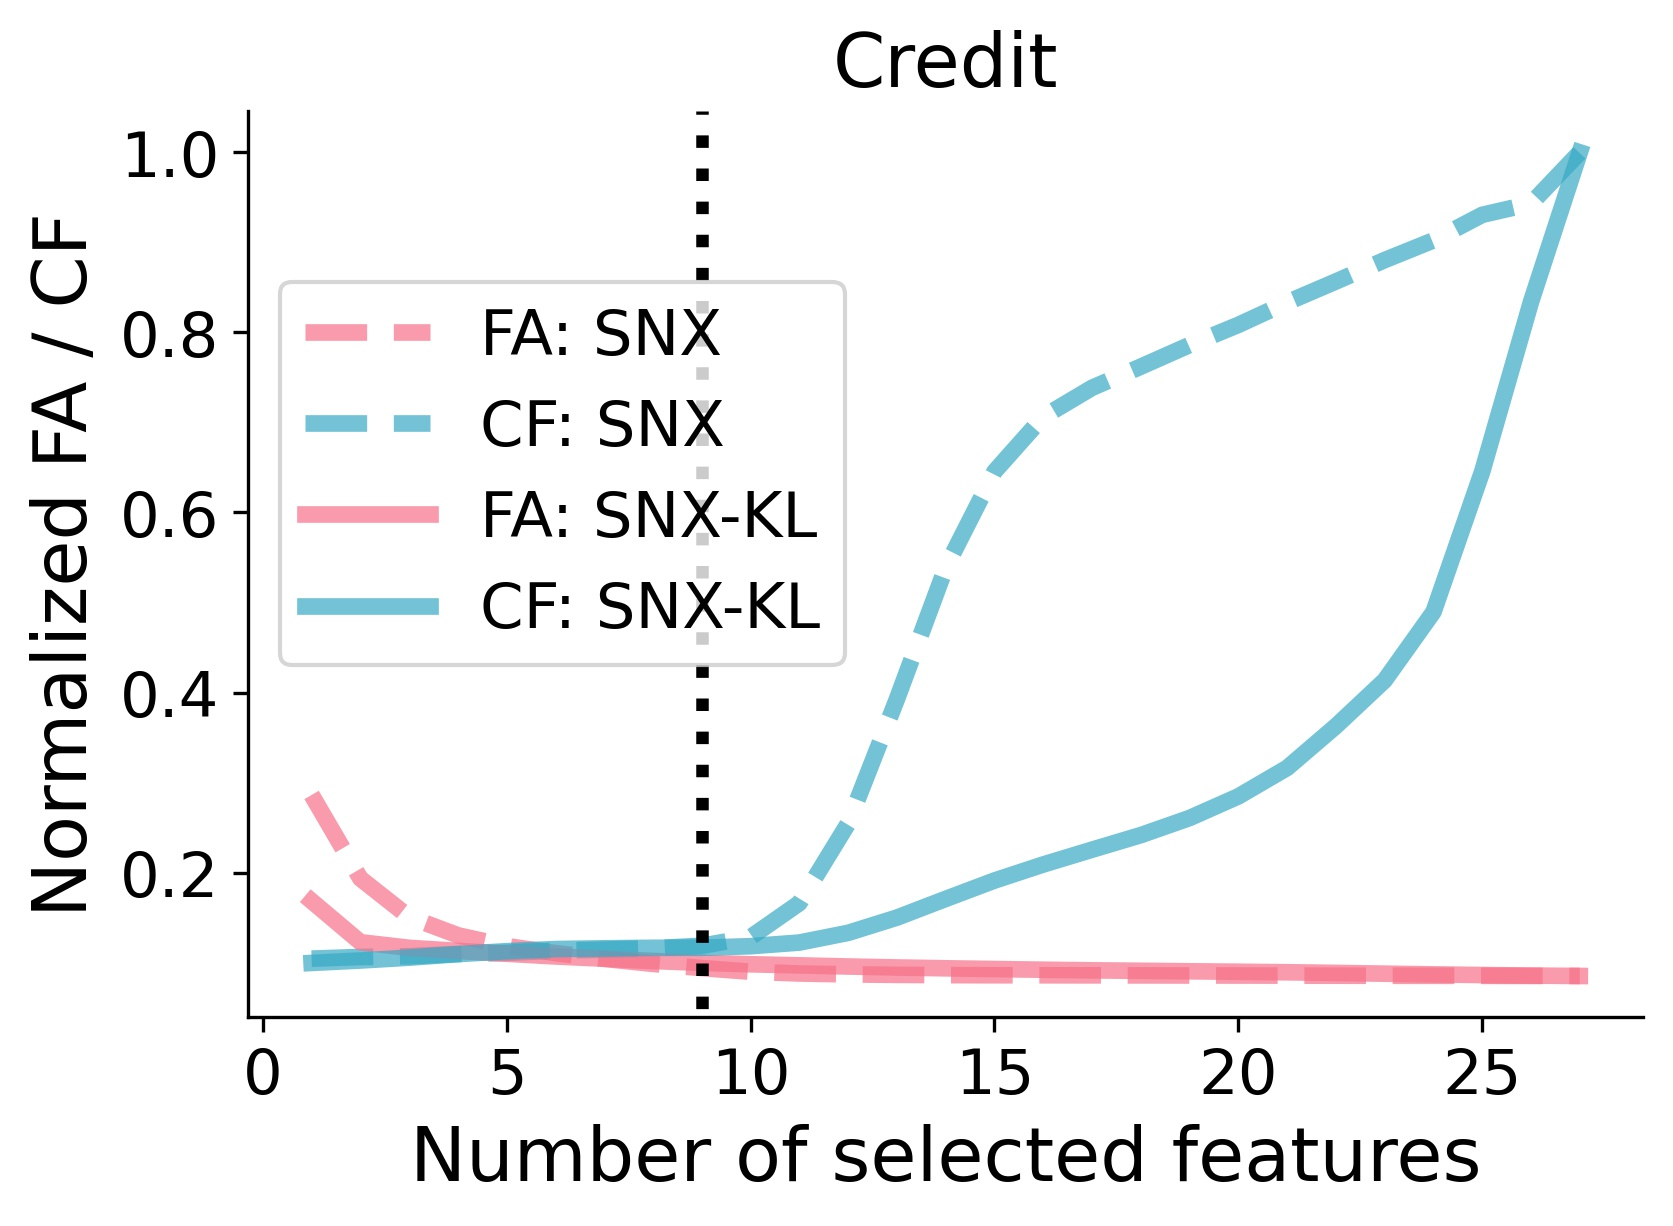}
\end{minipage}\\
\begin{minipage}{.15\textwidth}
    \includegraphics[width=\textwidth]{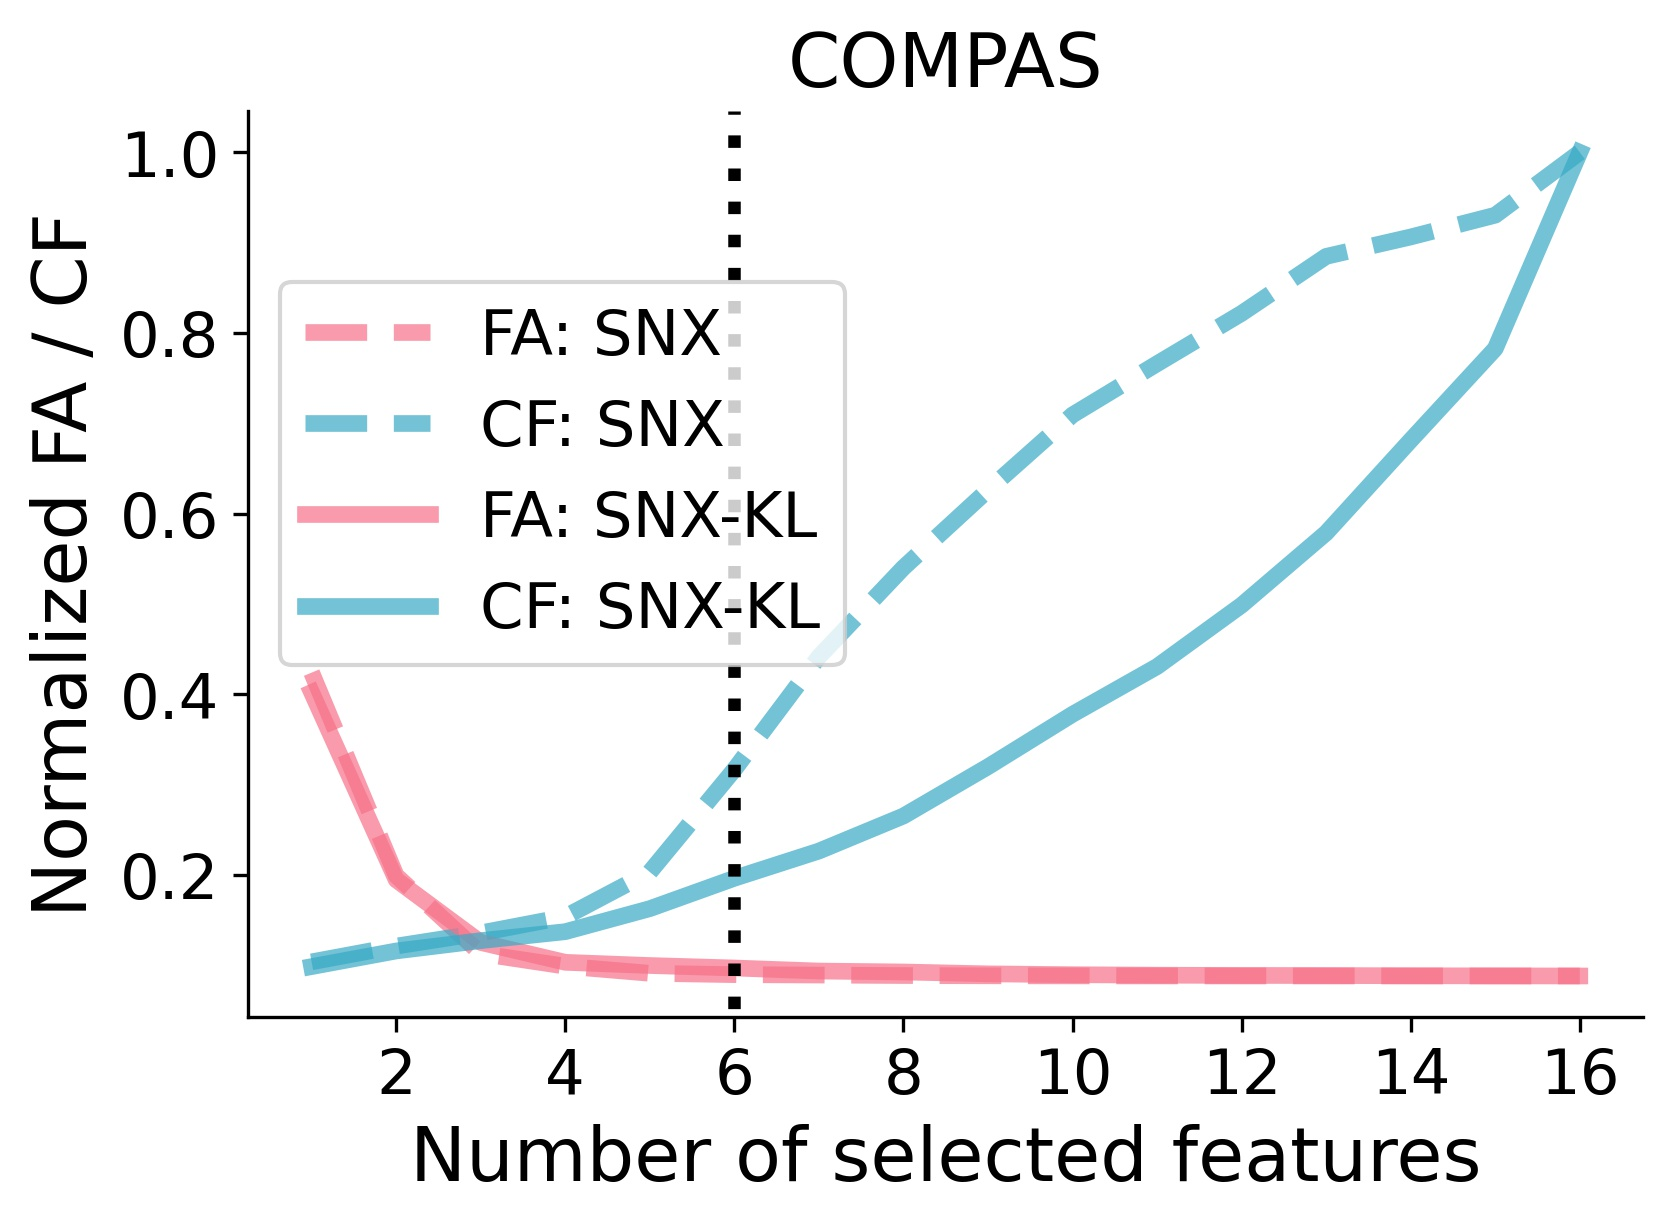}
\end{minipage}%
\begin{minipage}{.15\textwidth}
    \includegraphics[width=\textwidth]{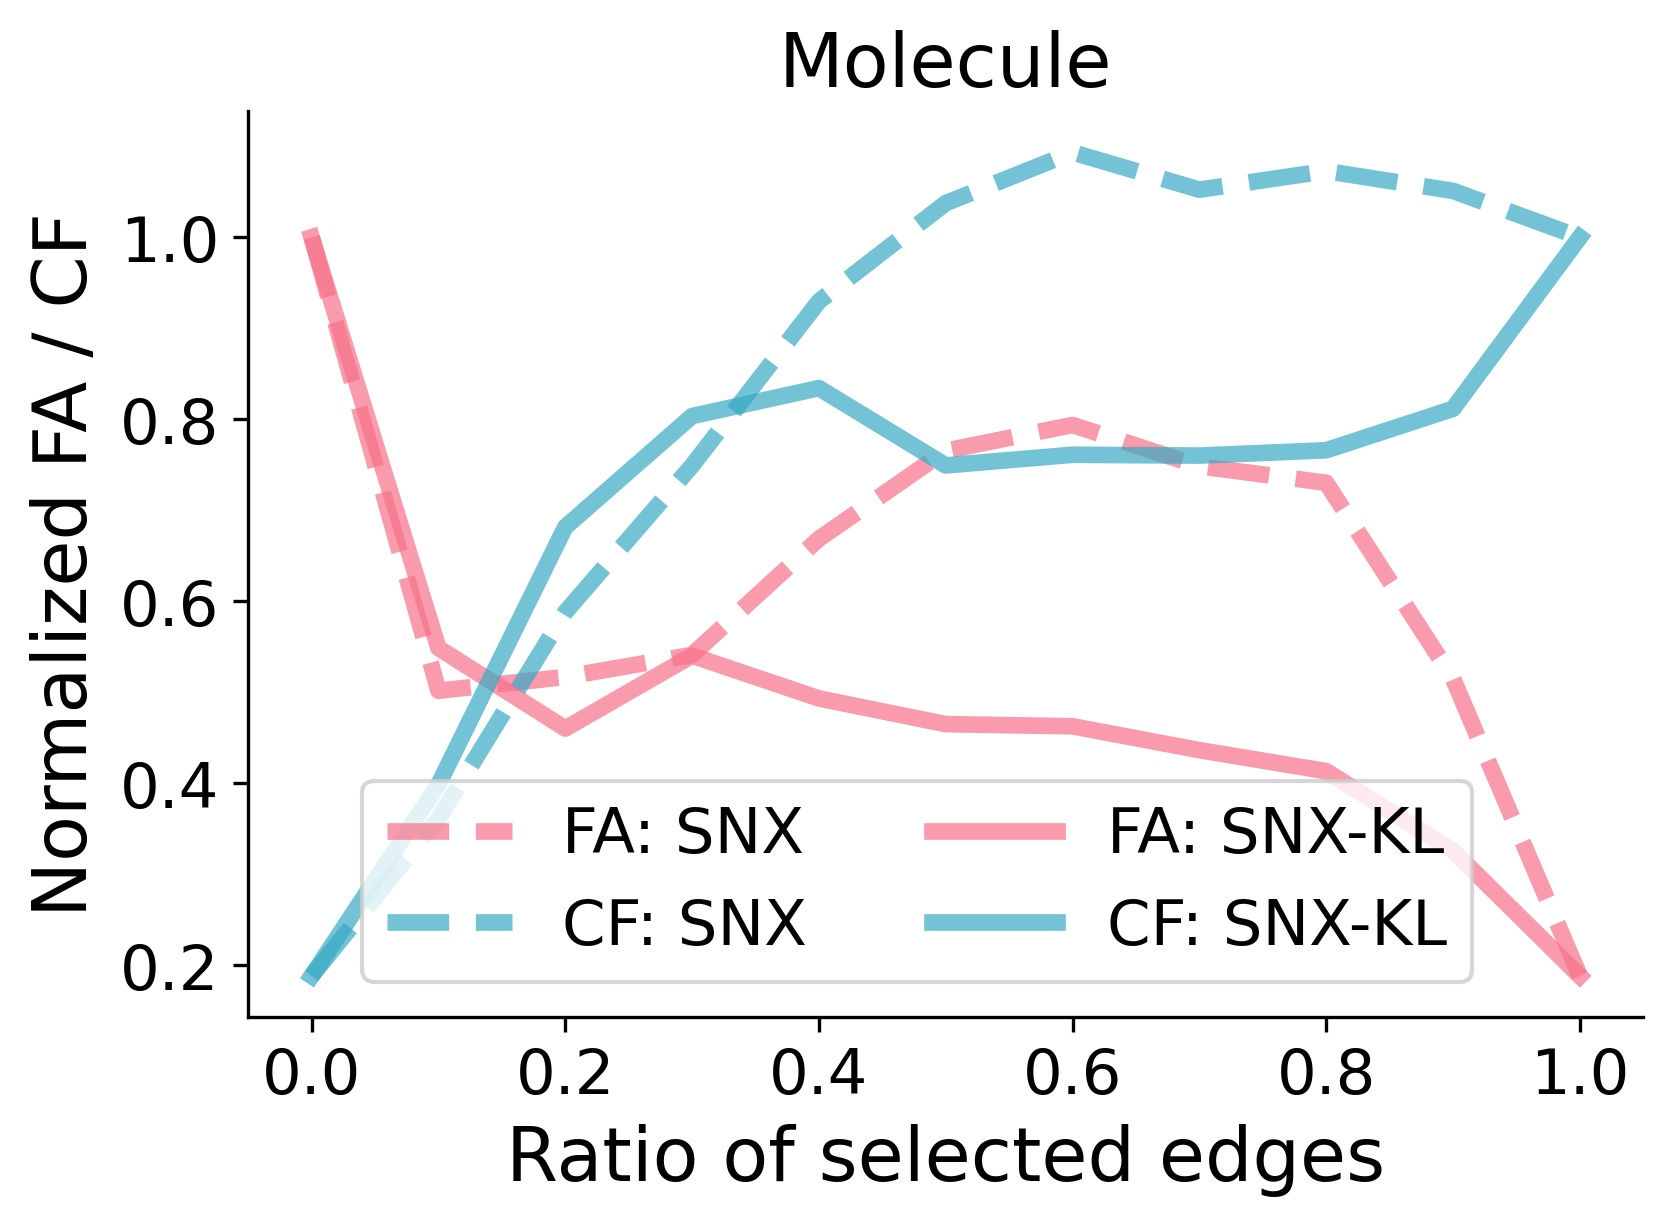}
\end{minipage}%
\begin{minipage}{.15\textwidth}
    \includegraphics[width=\textwidth]{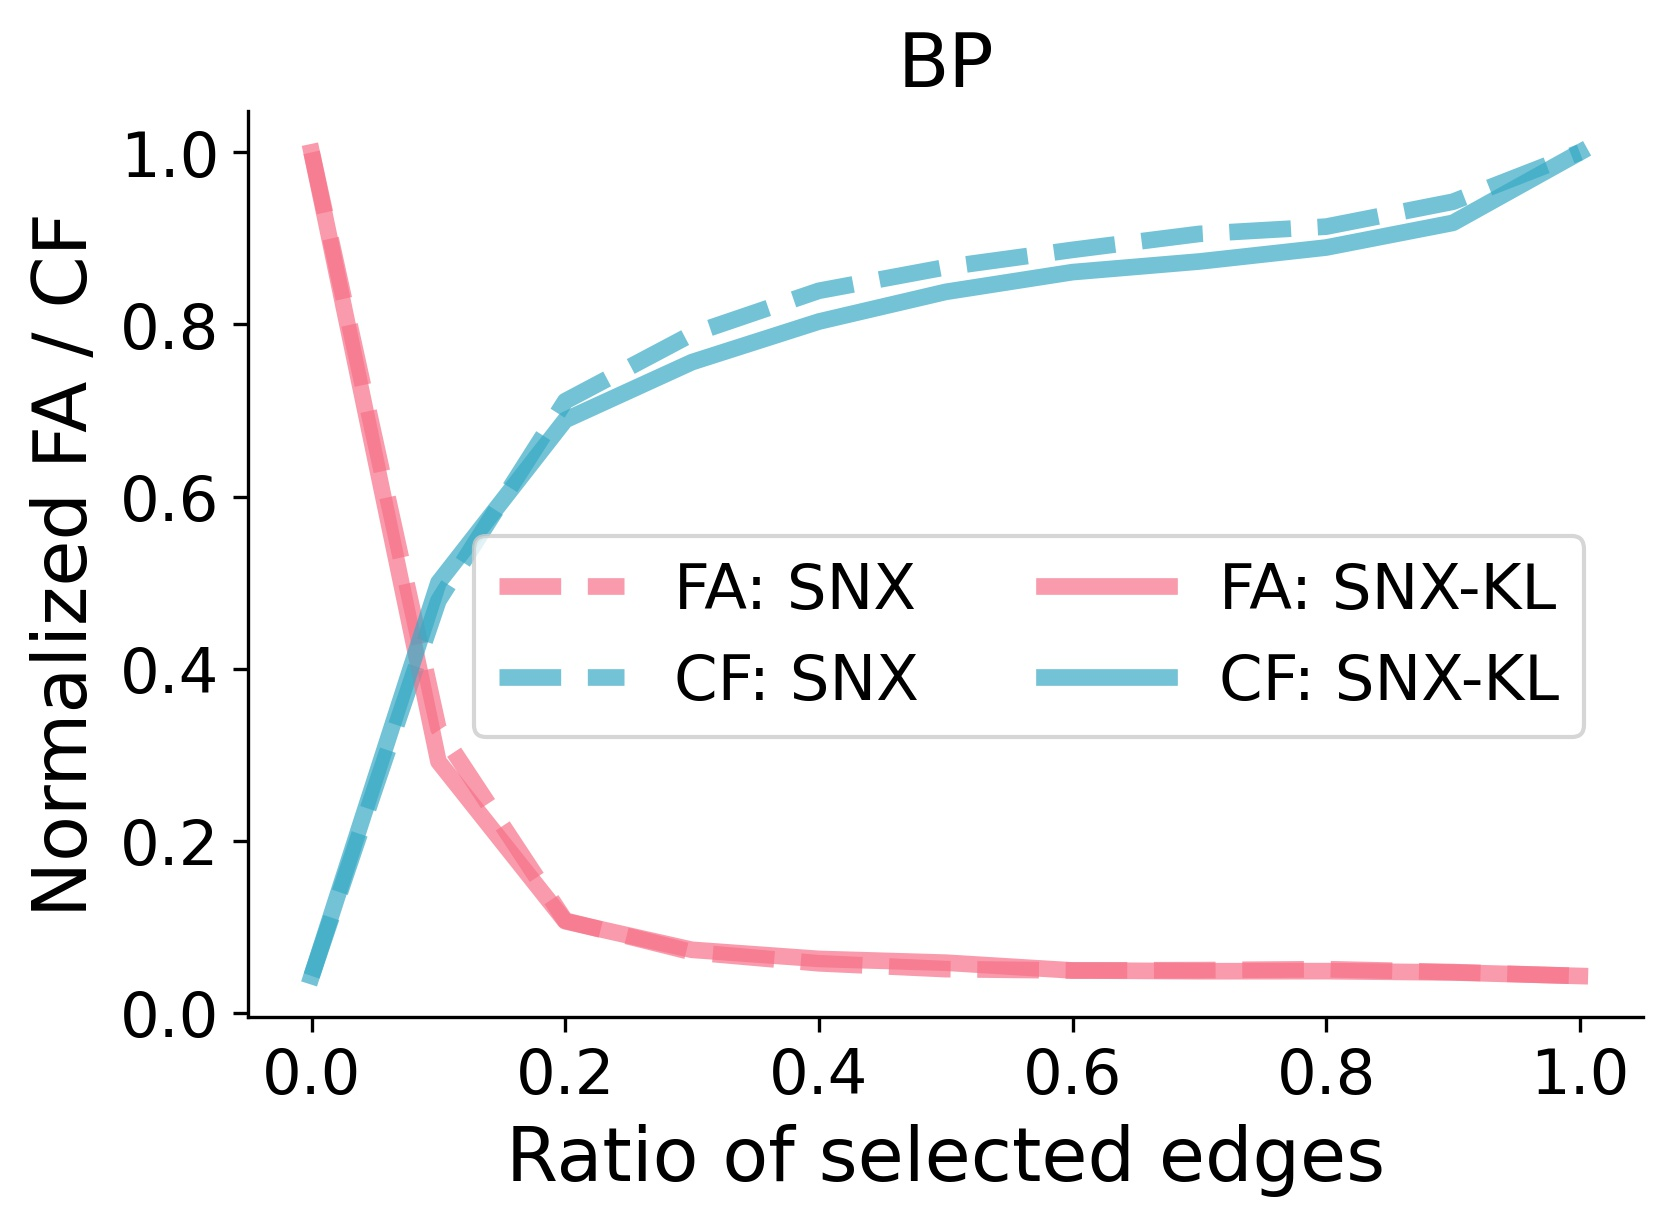}
\end{minipage}%
    \caption{\small The \textit{faithfulness} and \textit{counterfactual} of the local masks generated by SNX-KL and SNX, respectively,
    with different number/percentage of the selected features/edges.
    % \textcolor{blue}{Settings: It is a complete result of Figure 6 on all datasets.}
    }
    \label{fig:local_faithfulness}
\end{figure}

\begin{figure}[t]
    \centering
\begin{minipage}{.15\textwidth}
    \includegraphics[width=\textwidth]{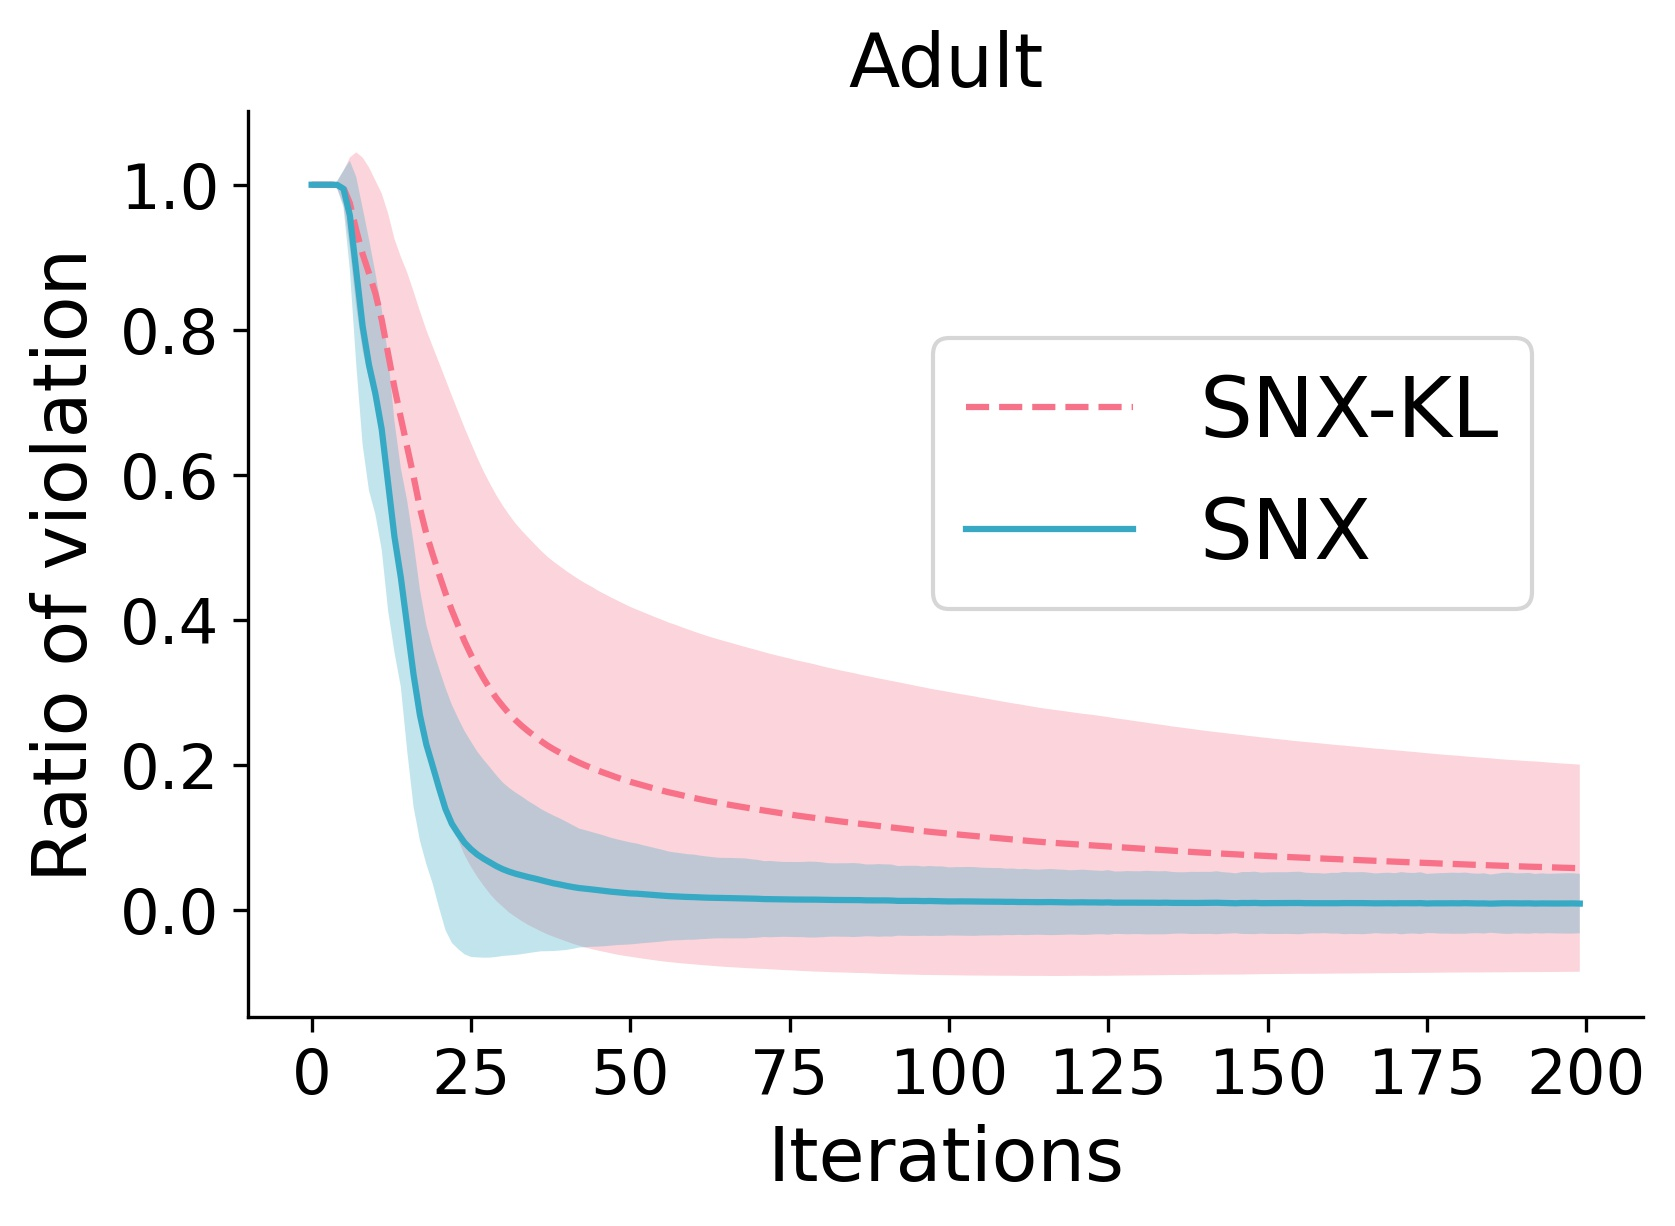}
\end{minipage}%
\begin{minipage}{.15\textwidth}
    \includegraphics[width=\textwidth]{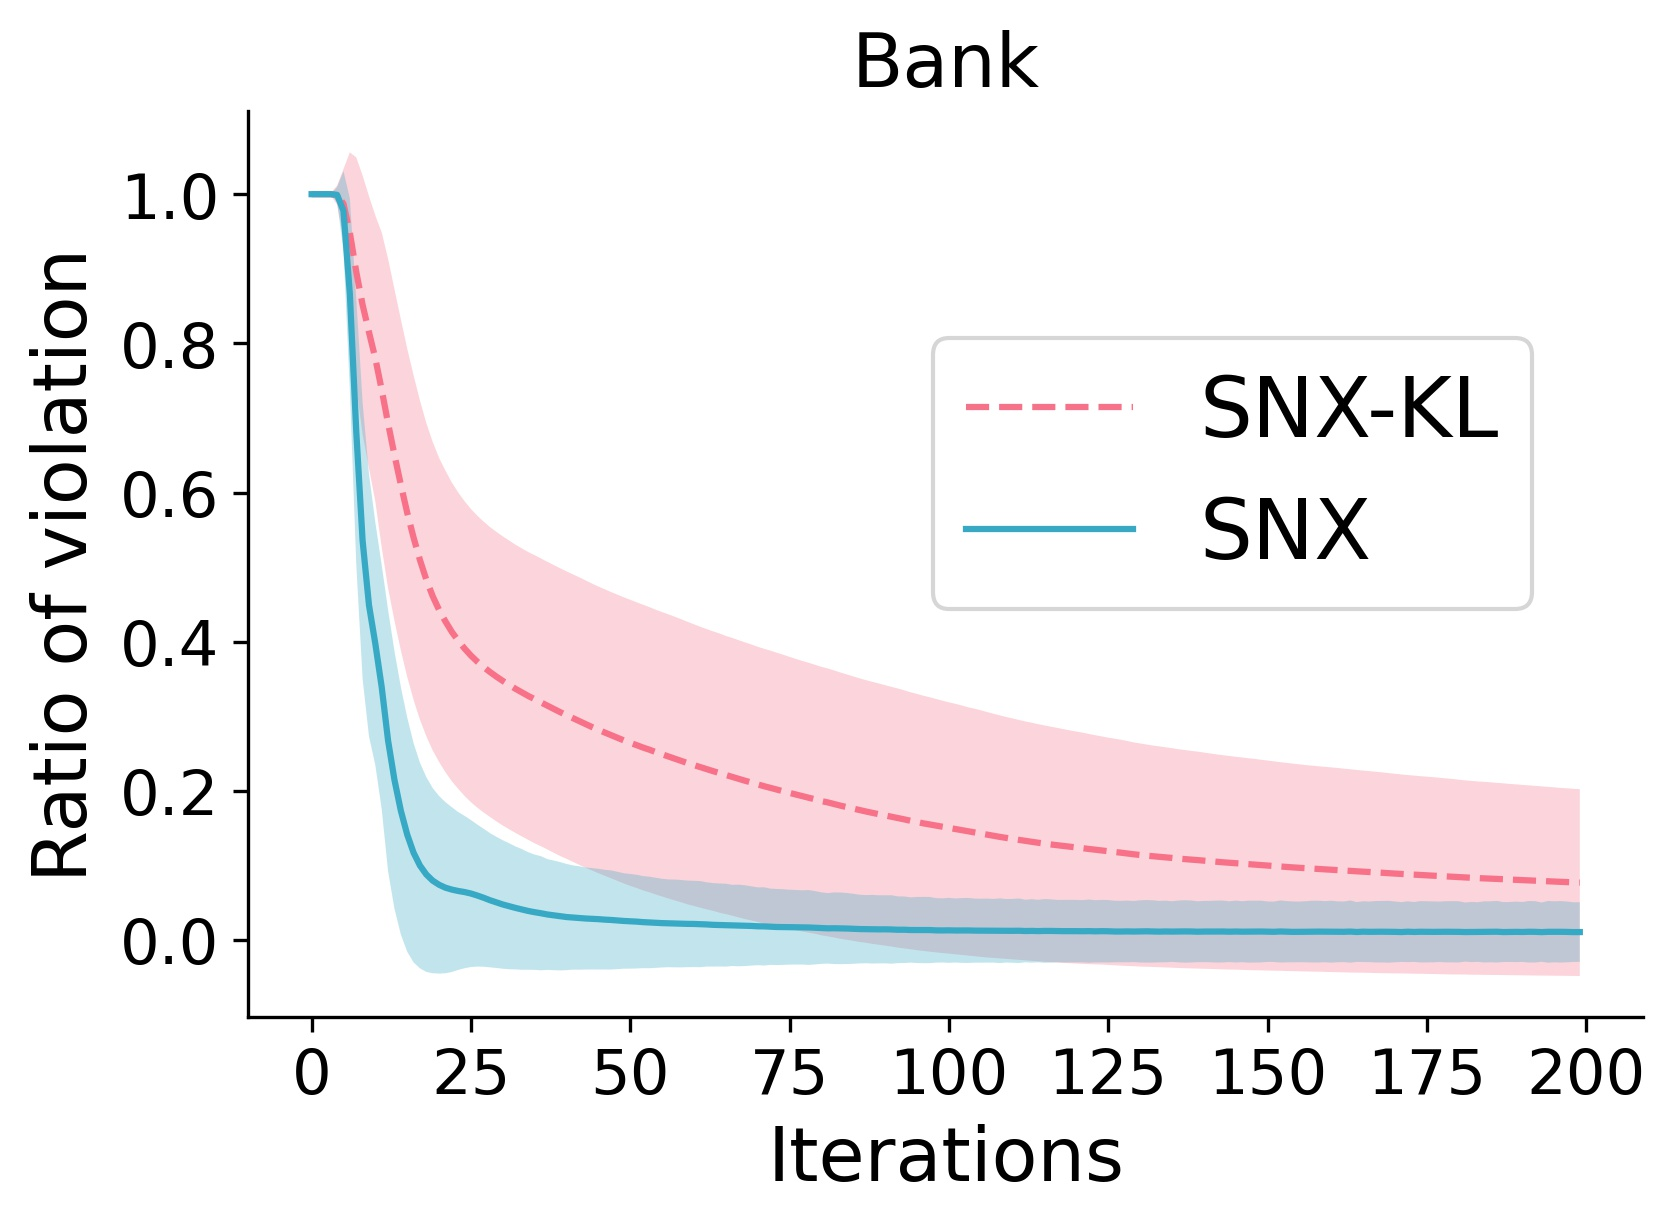}
\end{minipage}%
\begin{minipage}{.15\textwidth}
    \includegraphics[width=\textwidth]{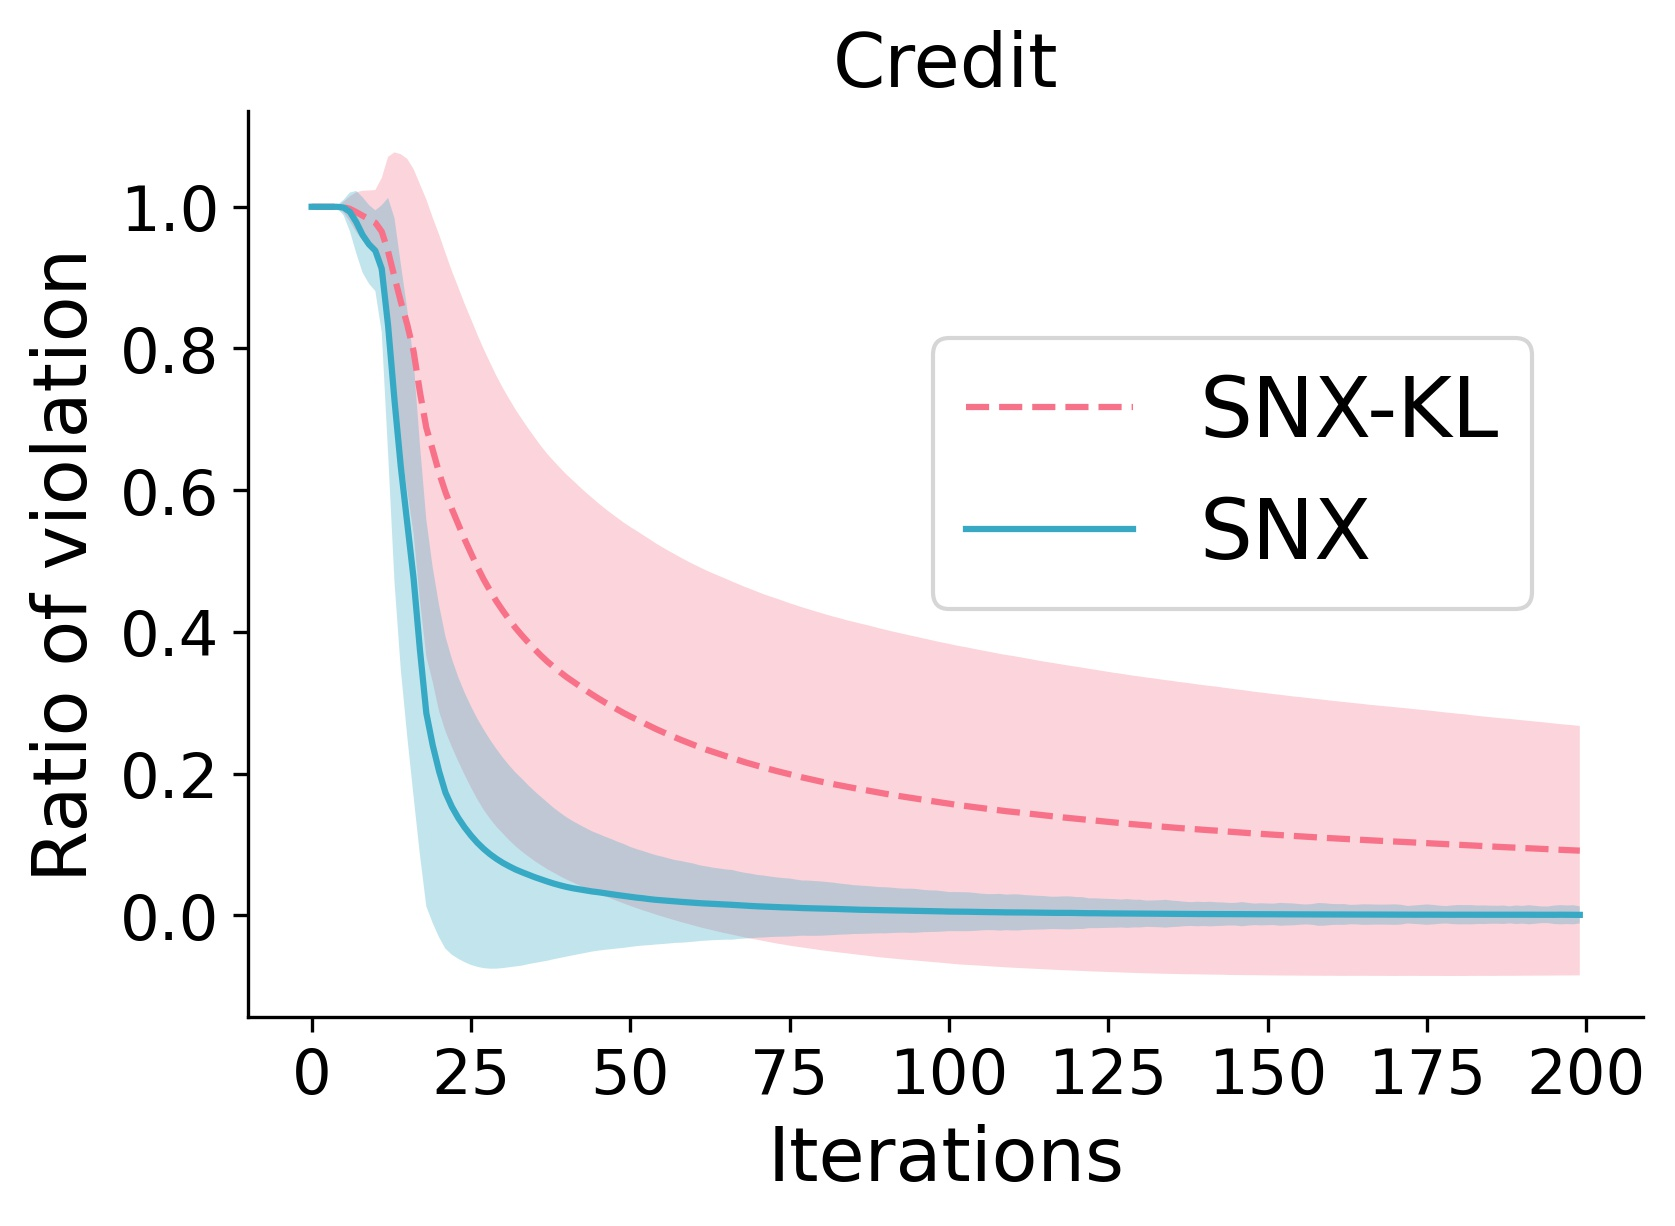}
\end{minipage}\\
\begin{minipage}{.15\textwidth}
    \includegraphics[width=\textwidth]{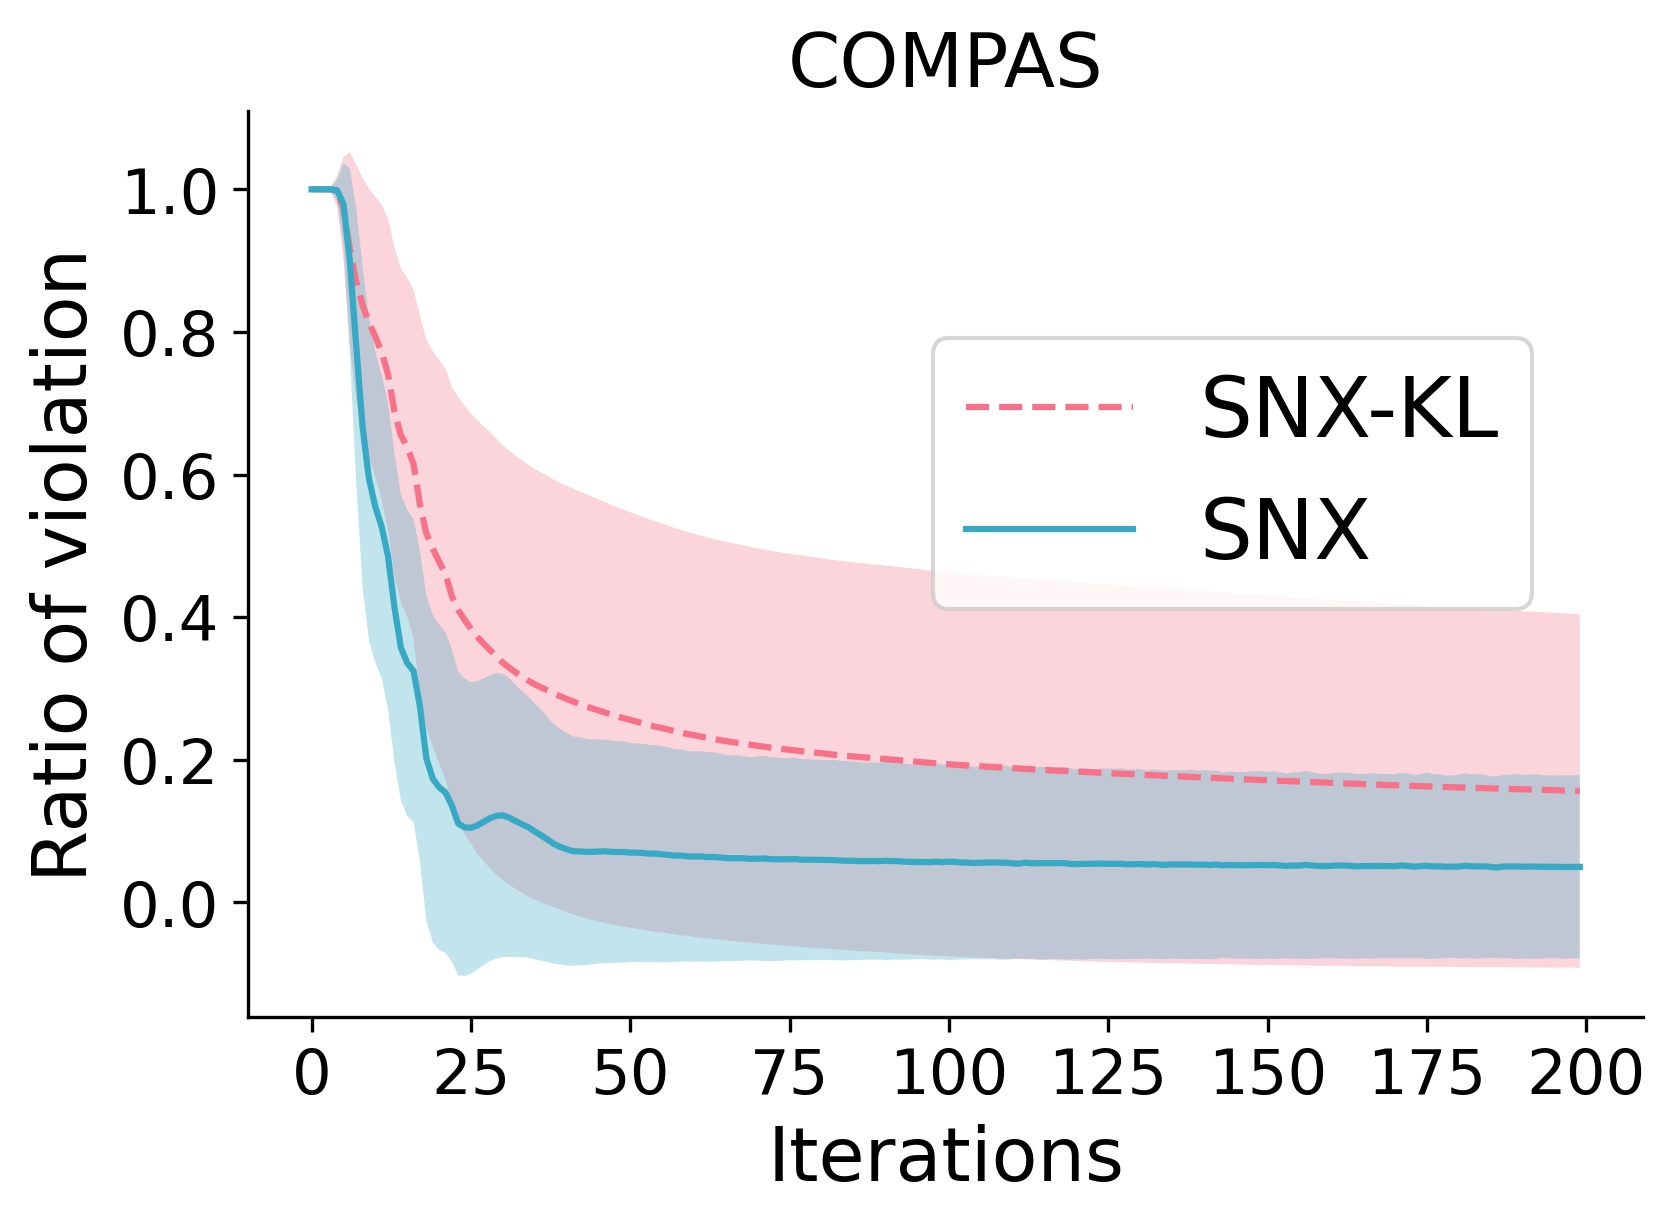}
\end{minipage}%
\begin{minipage}{.15\textwidth}
    \includegraphics[width=\textwidth]{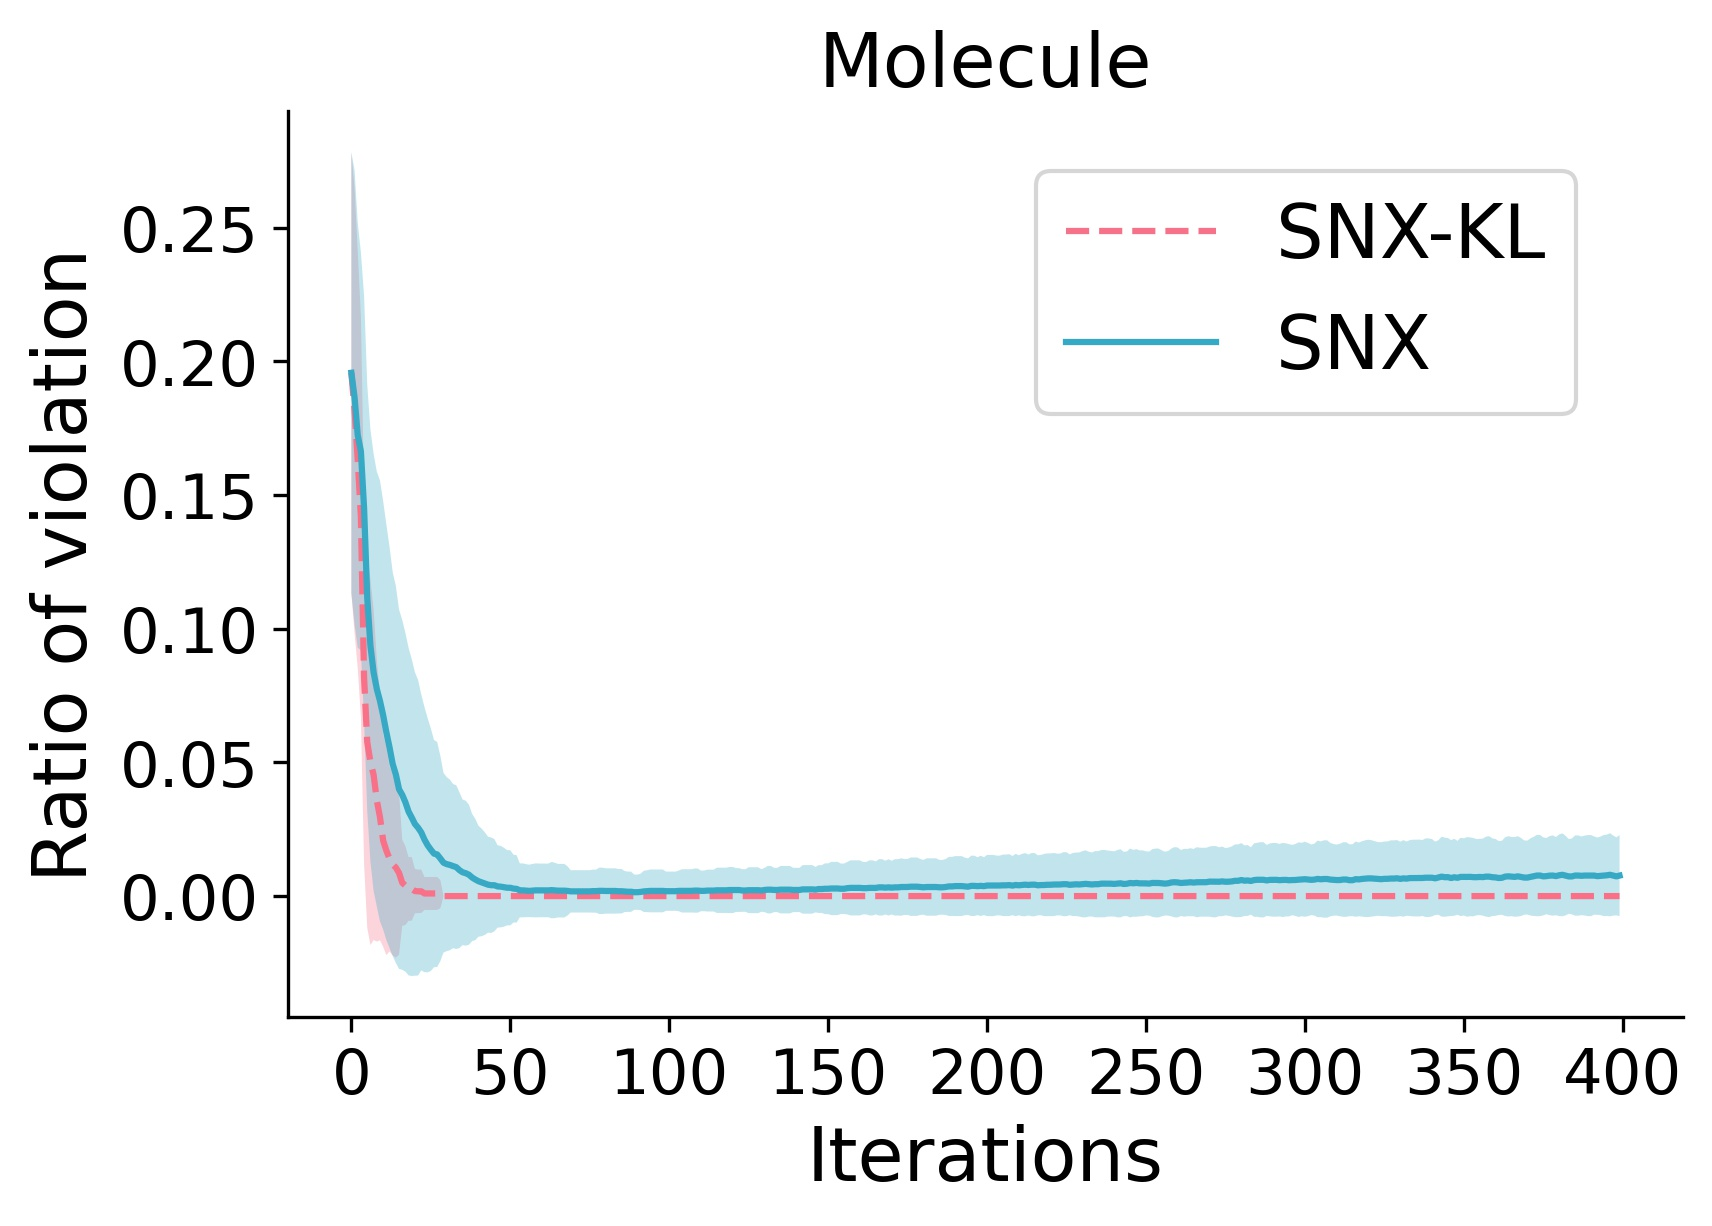}
\end{minipage}%
\begin{minipage}{.15\textwidth}
    \includegraphics[width=\textwidth]{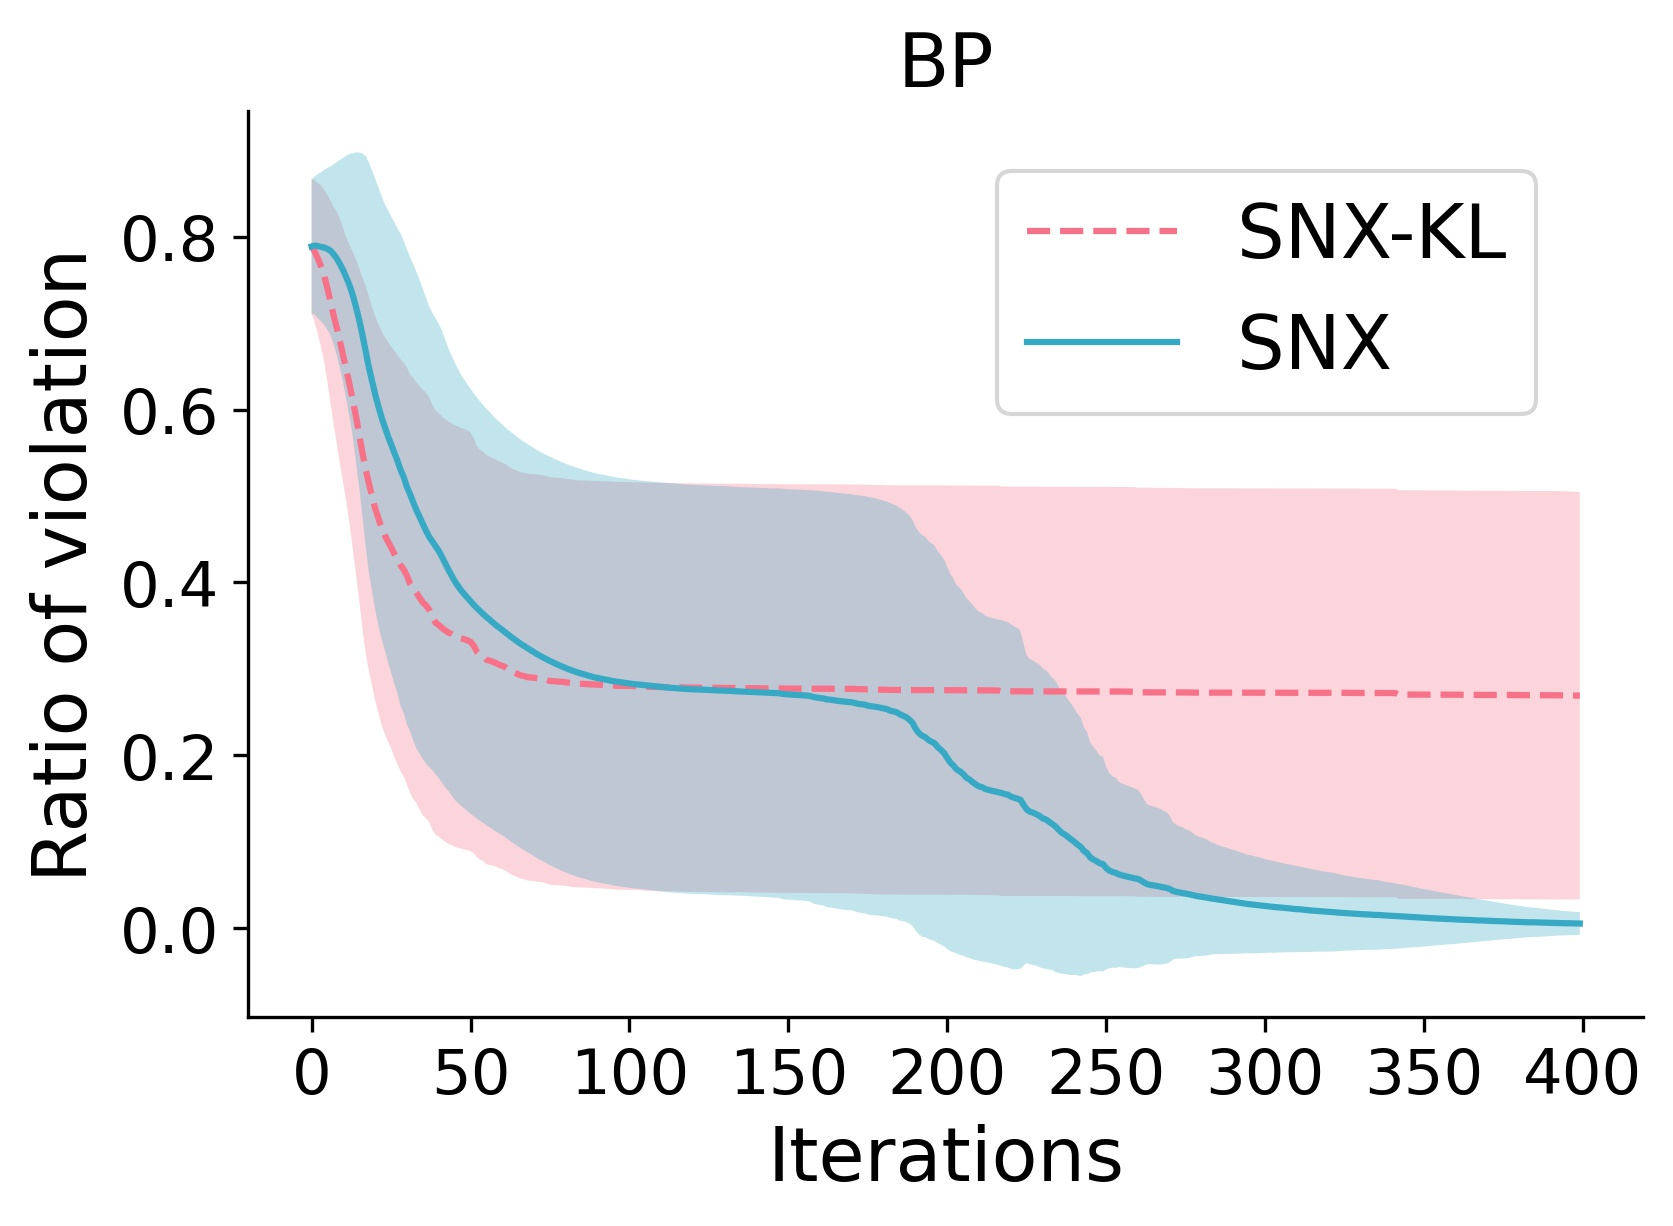}
\end{minipage}
    \caption{\small Comparing the ratio of instances breaking constraints in the first 200 iterations (in four tabular datasets) and 400 iterations (in two graph datasets) by using SNX-KL and SNX.
    % \textcolor{blue}{Settings: We record the intermediate local masks (float-type) and compare it with the fixed global masks (float-type), to see the ratio of violations during optimizations.
    % 'Ratio' here means: # of violations / # of constraints.}
    }
    \label{fig:kl-lag-supp}
\end{figure}

\begin{figure}[t]
\centering
\begin{minipage}{.15\textwidth}
\includegraphics[width=\textwidth]{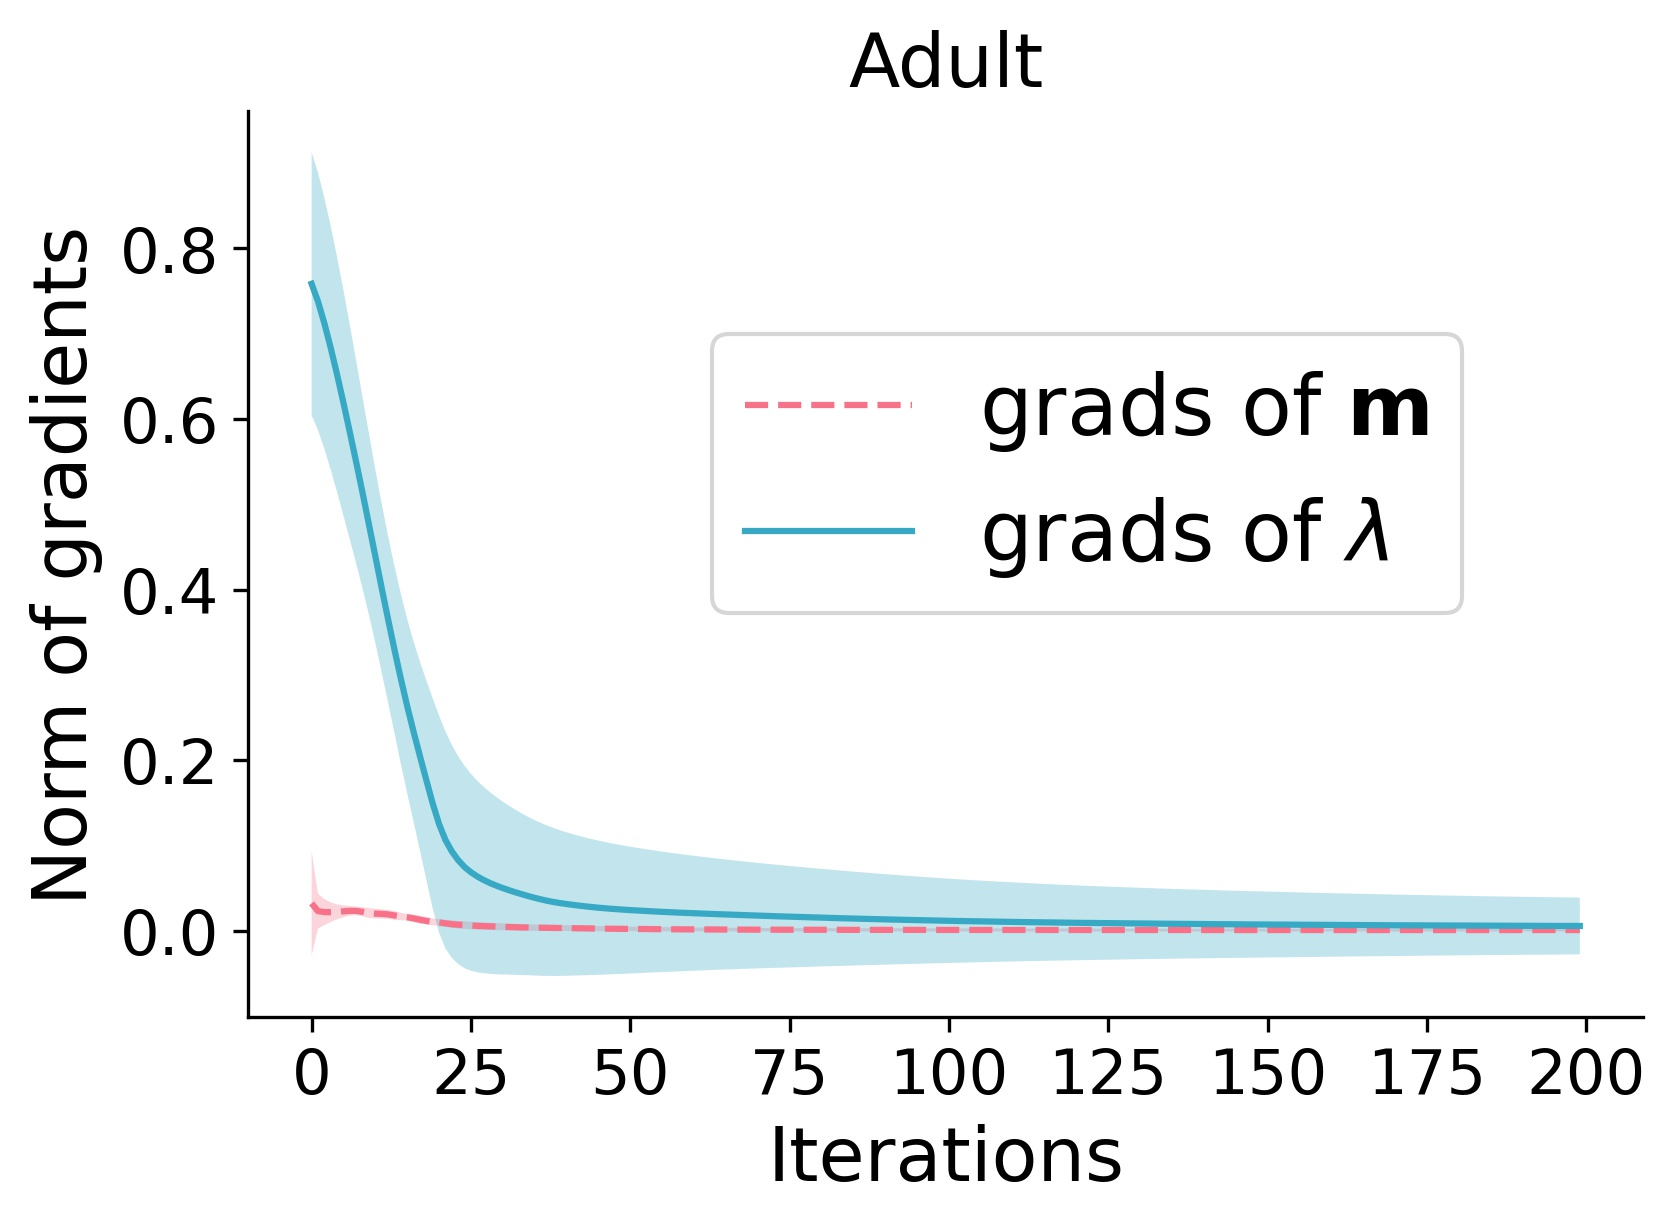}
\end{minipage}%
\begin{minipage}{.15\textwidth}
\includegraphics[width=\textwidth]{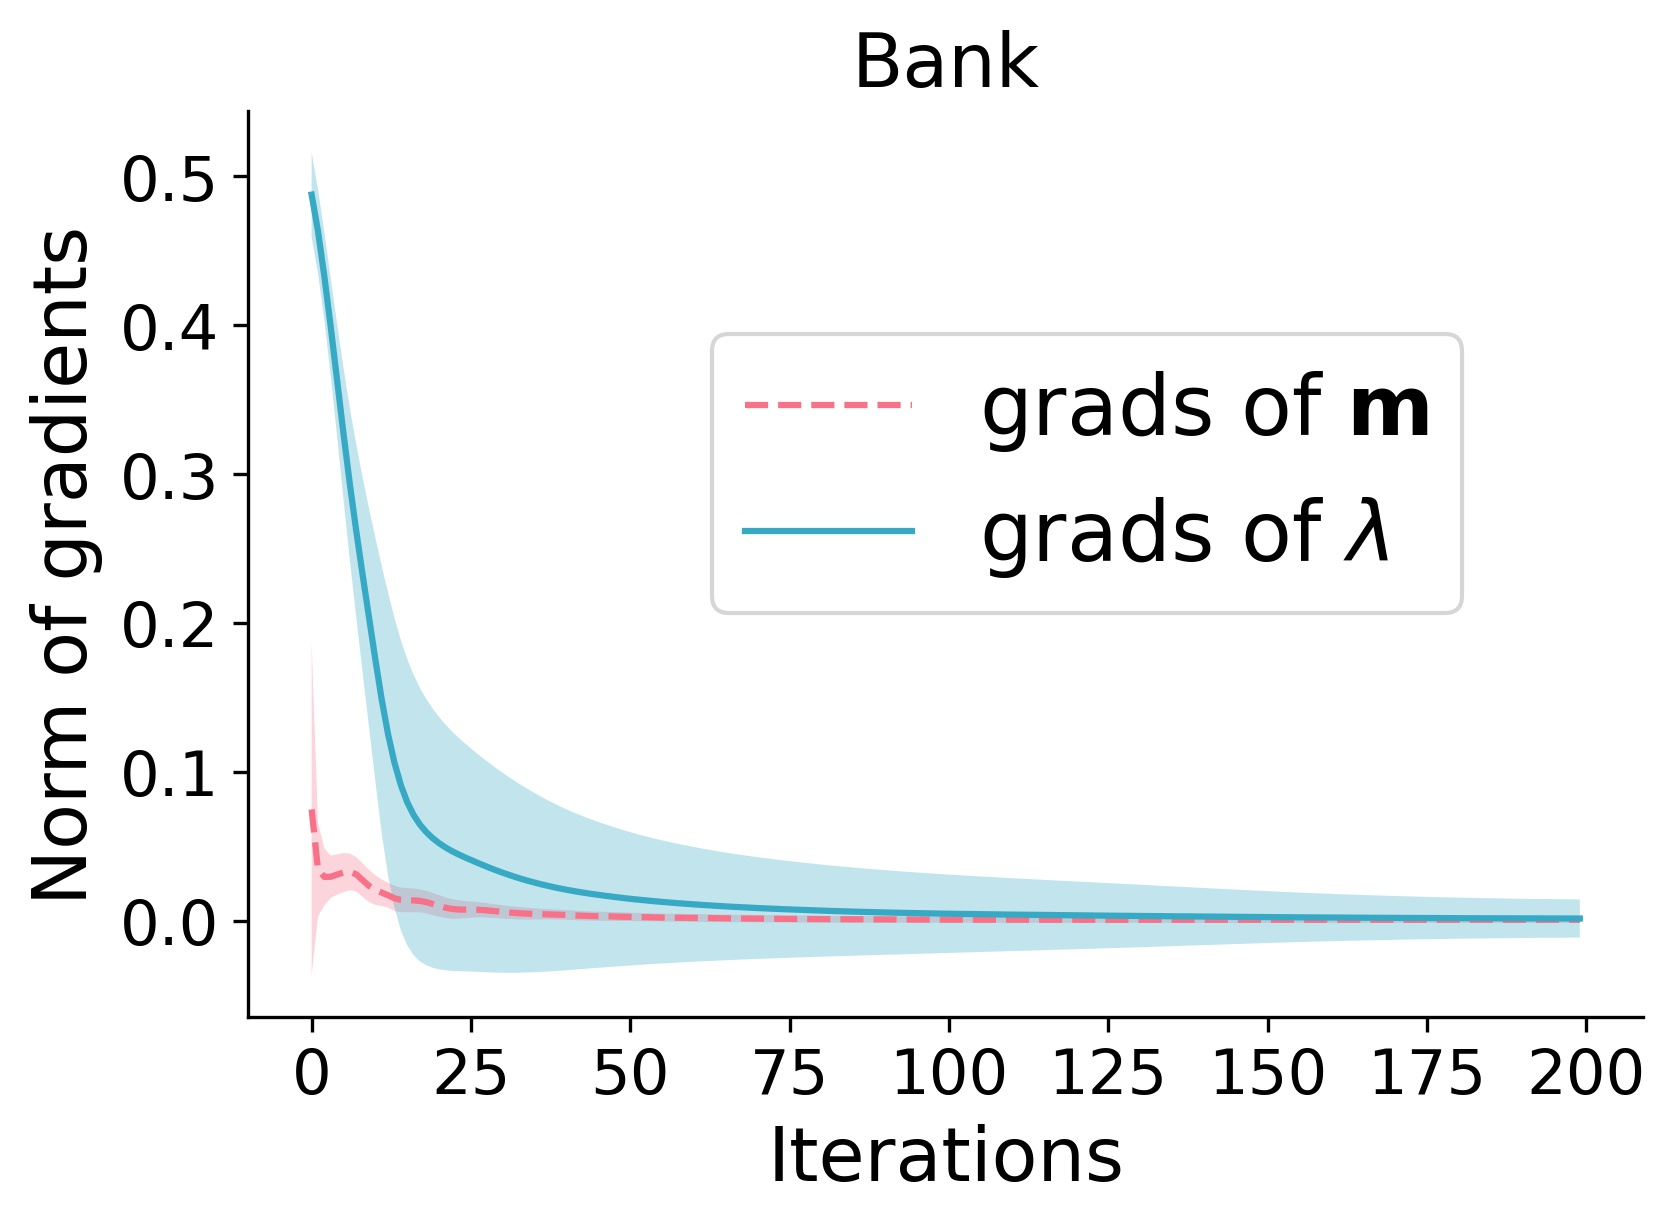}
\end{minipage}%
\begin{minipage}{.15\textwidth}
\includegraphics[width=\textwidth]{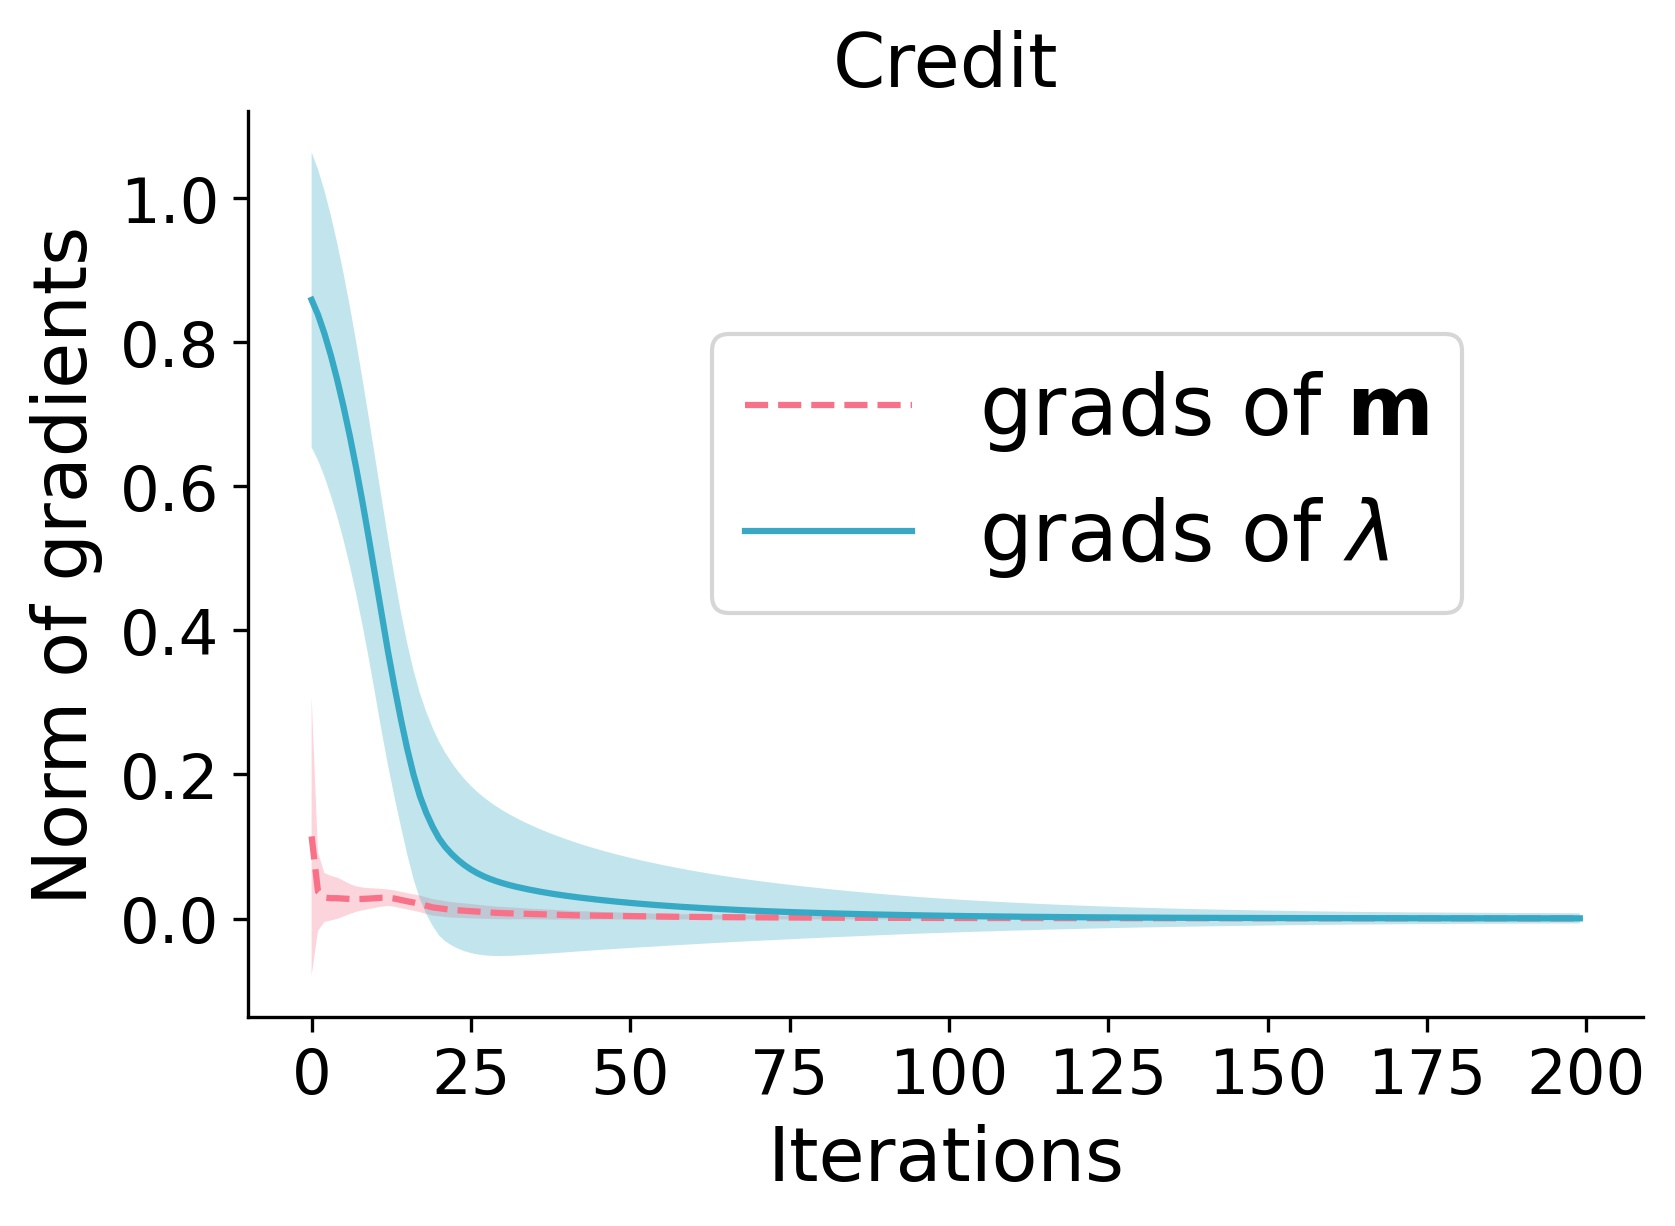}
\end{minipage}\\
\begin{minipage}{.15\textwidth}
\includegraphics[width=\textwidth]{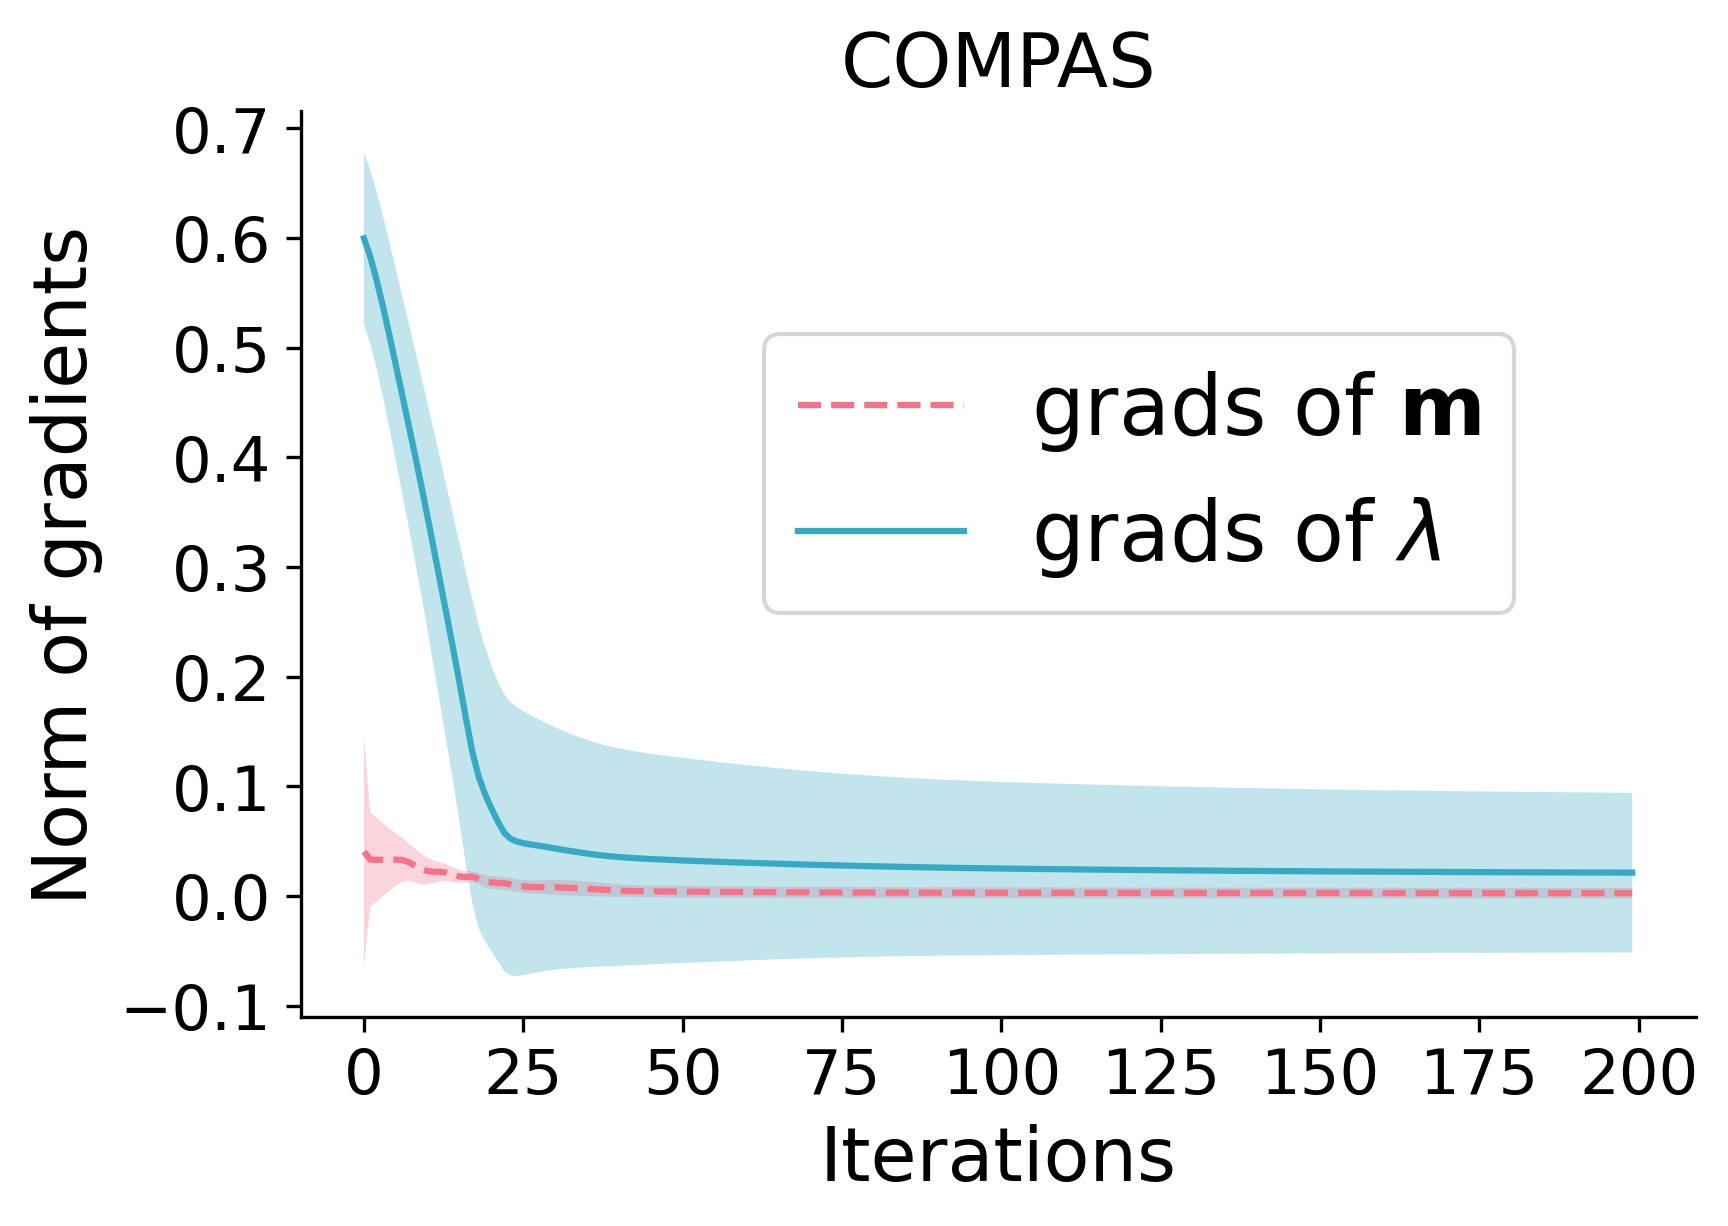}
\end{minipage}%
\begin{minipage}{.15\textwidth}
\includegraphics[width=\textwidth]{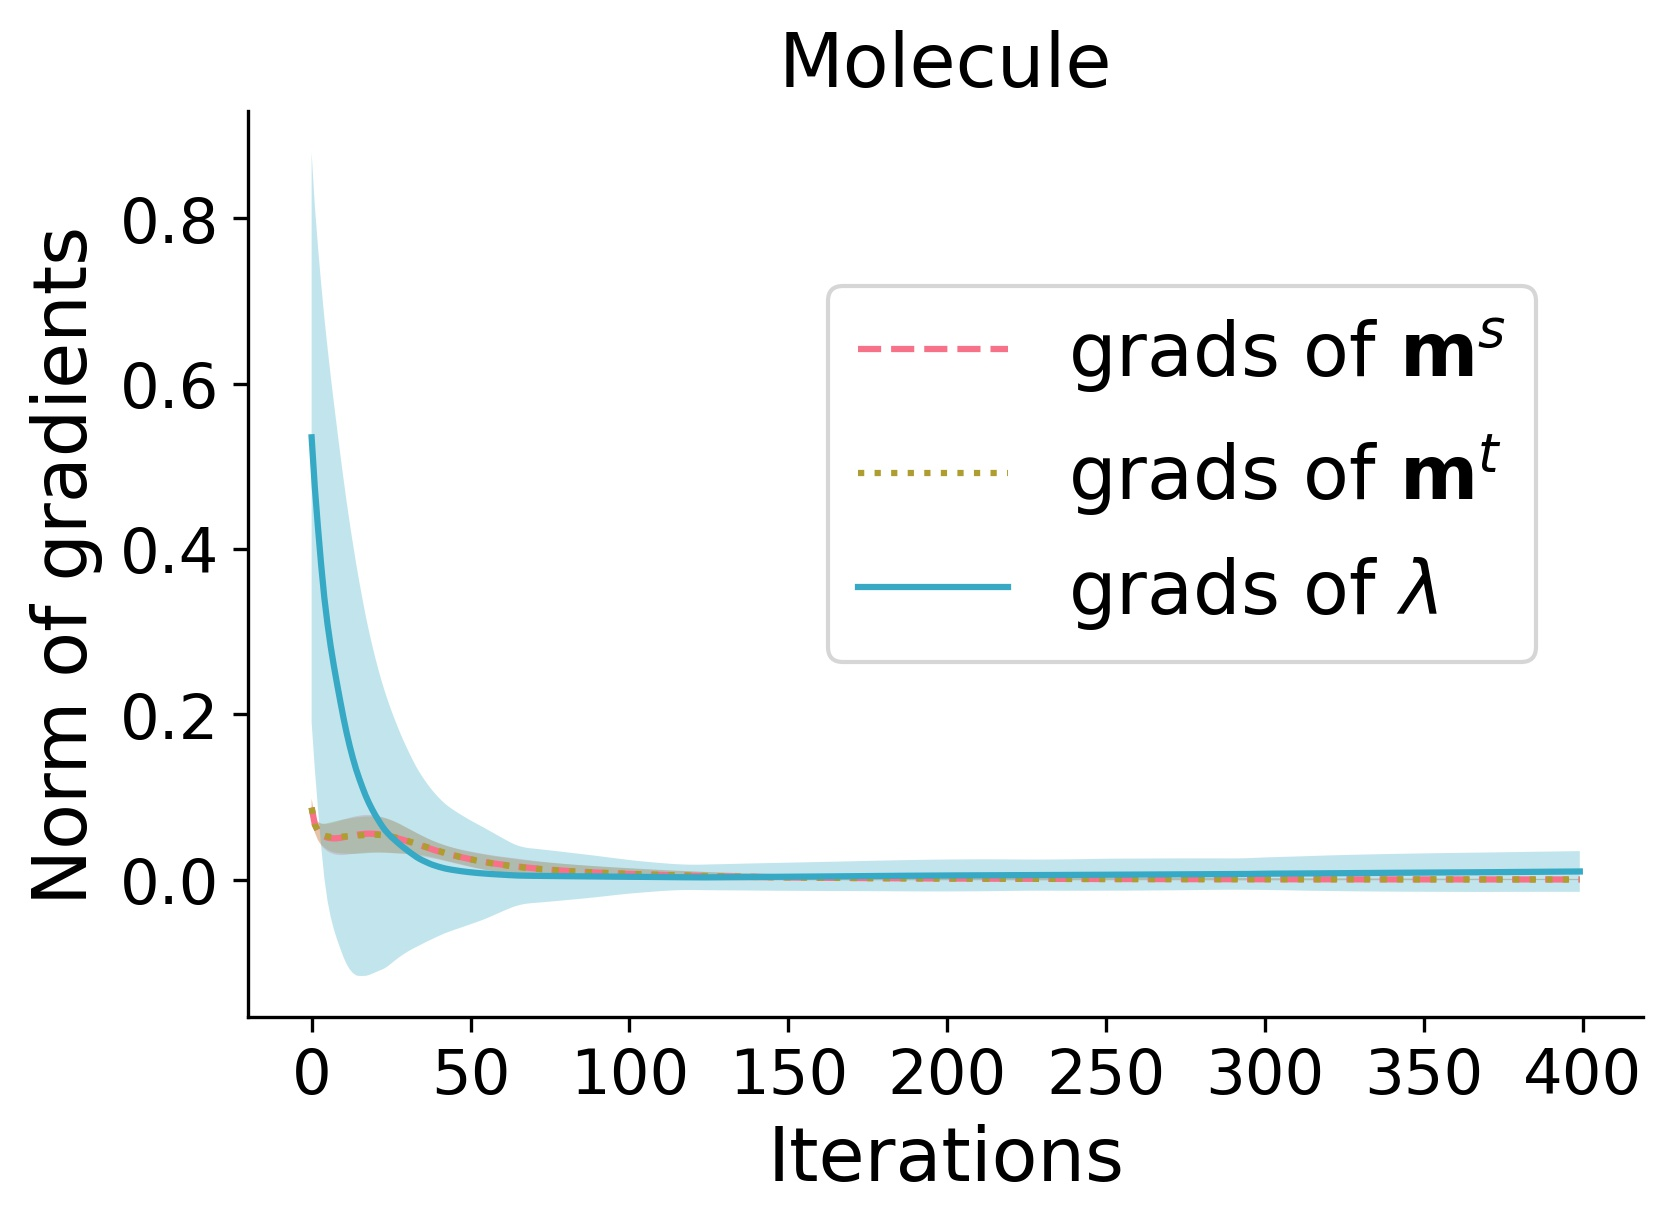}
\end{minipage}%
\begin{minipage}{.15\textwidth}
\includegraphics[width=\textwidth]{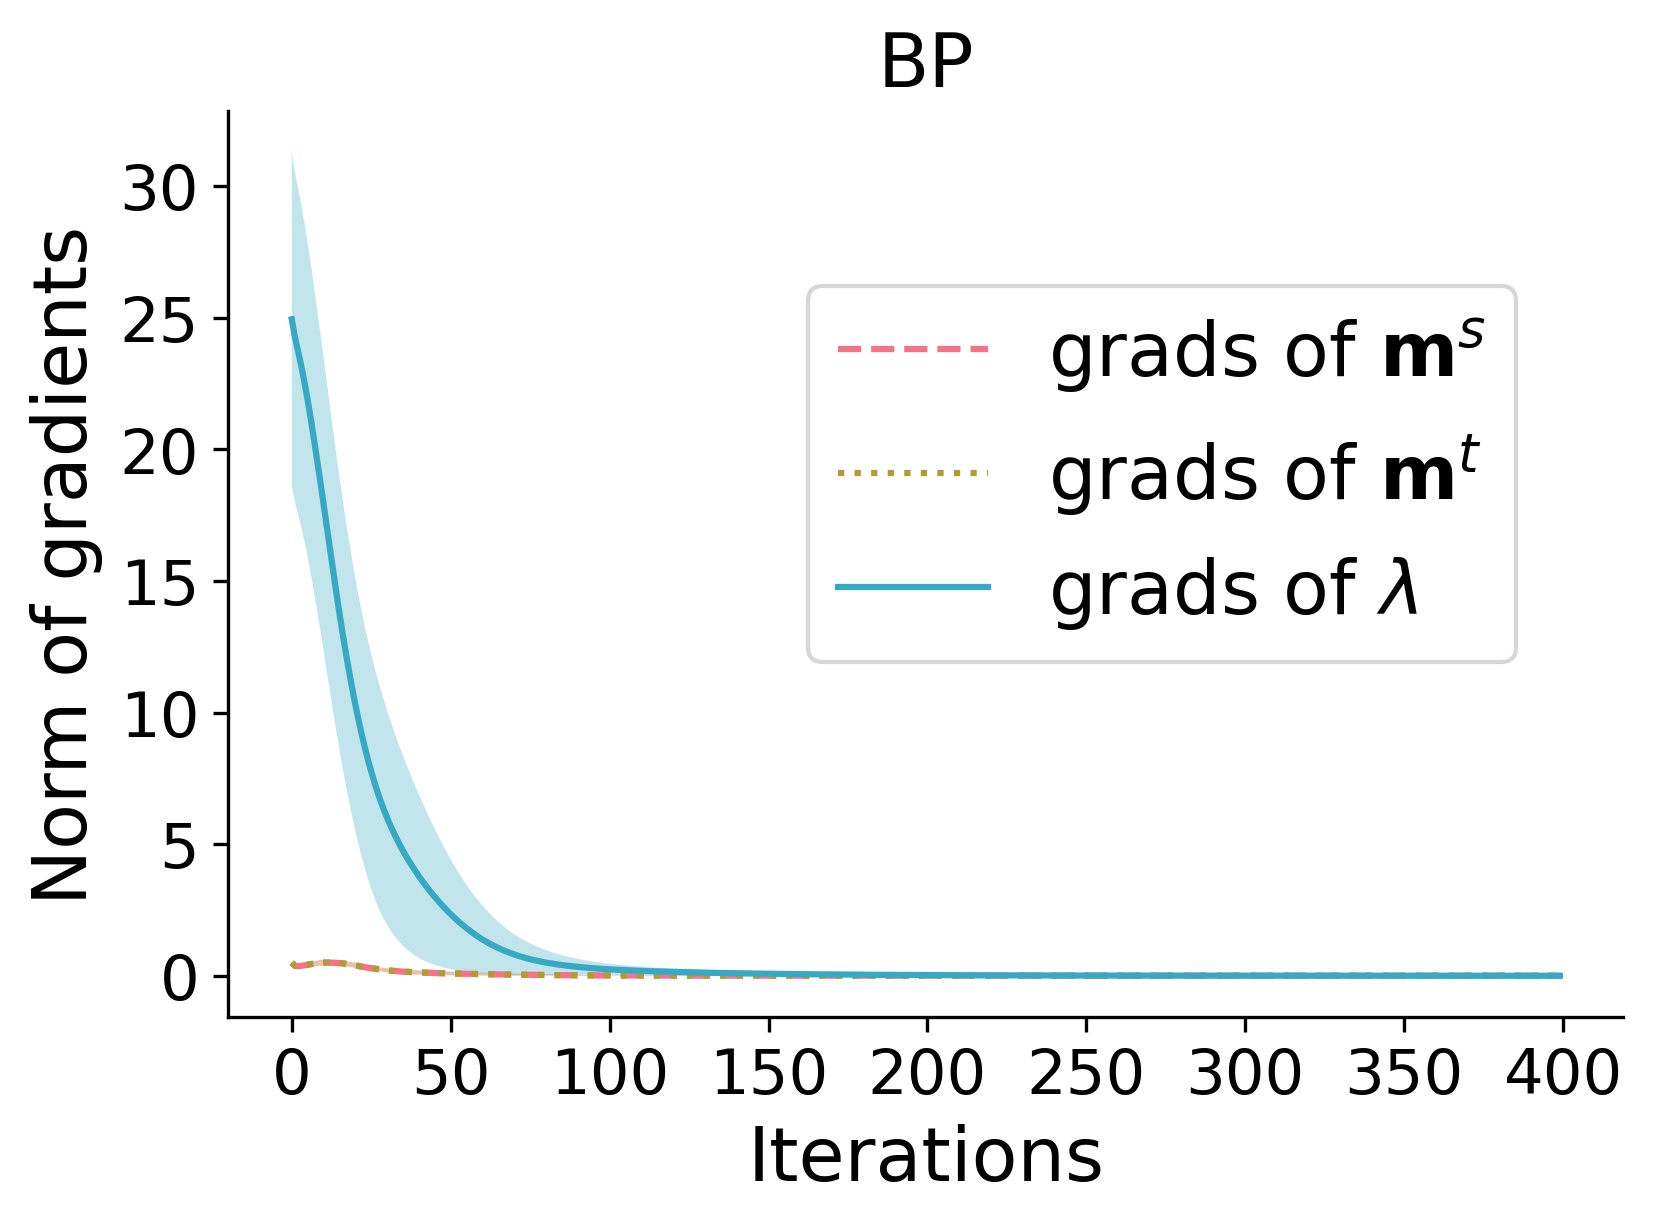}
\end{minipage}
\caption{\small It shows the trend of the norm of $\mathbf{m}$'s and $\boldsymbol{\lambda}$'s gradients during the optimization by Algorithm-\ref{alg:con_opt} in all datasets.
% and two graph datasets.
% \textcolor{blue}{Settings: It is a complete results of Figure 5 on all datasets.}
}
\label{fig:grads_complete}
\end{figure}

\begin{figure*}[!h]
    \scriptsize
    \centering
    \caption{\small The same case study as in Table~\ref{tab:simplified_case_study} with feature values given. 
    }
    \label{tab:case_study}
    \begin{tabular}{c | c | c c c c c c c c c c}
        \toprule
        \multicolumn{2}{c}{\textbf{Adult}} 
        % \textbf{Adult} 
        & Workclass & Race & Education & Age & Hours/week & Marital Status & Occupation & Relationship & Sex & Above/below 50k \\
        \midrule
        \multirow{3}{*}{Reference 1} 
        & SM
        & \cellcolor{red!75} Private 
        & \cellcolor{red!15} White 
        & \cellcolor{red!15} HS-grad 
        & \cellcolor{red!75} 36 
        & \cellcolor{red!45} 40 
        & \cellcolor{red!15} Divorced 
        & \cellcolor{red!45} Craft-repair 
        & \cellcolor{red!75} Unmarried 
        & \cellcolor{red!45} Male 
        & Below \\
        & SNX-UC
        & \cellcolor{red!75} Private 
        & \cellcolor{red!15} White 
        & \cellcolor{red!15} HS-grad 
        & \cellcolor{red!45} 36 
        & \cellcolor{red!75} 40 
        & \cellcolor{red!45} Divorced 
        & \cellcolor{red!45} Craft-repair 
        & \cellcolor{red!75} Unmarried 
        & \cellcolor{red!15} Male 
        & Below \\
        & SNX
        & \cellcolor{red!75} Private 
        & \cellcolor{red!15} White 
        & \cellcolor{red!45} HS-grad 
        & \cellcolor{red!15} 36 
        & \cellcolor{red!75} 40 
        & \cellcolor{red!45} Divorced 
        & \cellcolor{red!75} Craft-repair 
        & \cellcolor{red!15} Unmarried 
        & \cellcolor{red!15} Male 
        & Below \\
        \midrule
        Query 
        & SNX-global
        & \cellcolor{blue!75} \textbf{Private} 
        & \cellcolor{blue!15} Black 
        & \cellcolor{blue!75} \textbf{Bachelors} 
        & \cellcolor{blue!15} 36 
        & \cellcolor{blue!75} \textbf{40} 
        & \cellcolor{blue!45} Never 
        & \cellcolor{blue!75} \textbf{Sales }
        & \cellcolor{blue!45} Unmarried 
        & \cellcolor{blue!15} Female 
        & Below \\
        \midrule
        \multirow{3}{*}{Reference 2} 
        & SNX
        & \cellcolor{red!75} Federal-gov 
        & \cellcolor{red!15} White 
        & \cellcolor{red!15} College
        & \cellcolor{red!15} 46
        & \cellcolor{red!75} 80 
        & \cellcolor{red!45} Married 
        & \cellcolor{red!75} Adm-clerical 
        & \cellcolor{red!45} Husband 
        & \cellcolor{red!15} Male 
        & Above \\
        & SNX-UC
        & \cellcolor{red!75} Federal-gov 
        & \cellcolor{red!15} White 
        & \cellcolor{red!15} College
        & \cellcolor{red!45} 46
        & \cellcolor{red!45} 80 
        & \cellcolor{red!75} Married 
        & \cellcolor{red!75} Adm-clerical 
        & \cellcolor{red!45} Husband 
        & \cellcolor{red!15} Male 
        & Above \\
        & SM 
        & \cellcolor{red!45} Federal-gov 
        & \cellcolor{red!75} White 
        & \cellcolor{red!15} College
        & \cellcolor{red!45} 46
        & \cellcolor{red!75} 80 
        & \cellcolor{red!15} Married 
        & \cellcolor{red!75} Adm-clerical 
        & \cellcolor{red!45} Husband 
        & \cellcolor{red!15} Male 
        & Above \\
        \bottomrule
    \end{tabular}

    \centering
\begin{minipage}{.2\textwidth}
    \includegraphics[width=\textwidth]{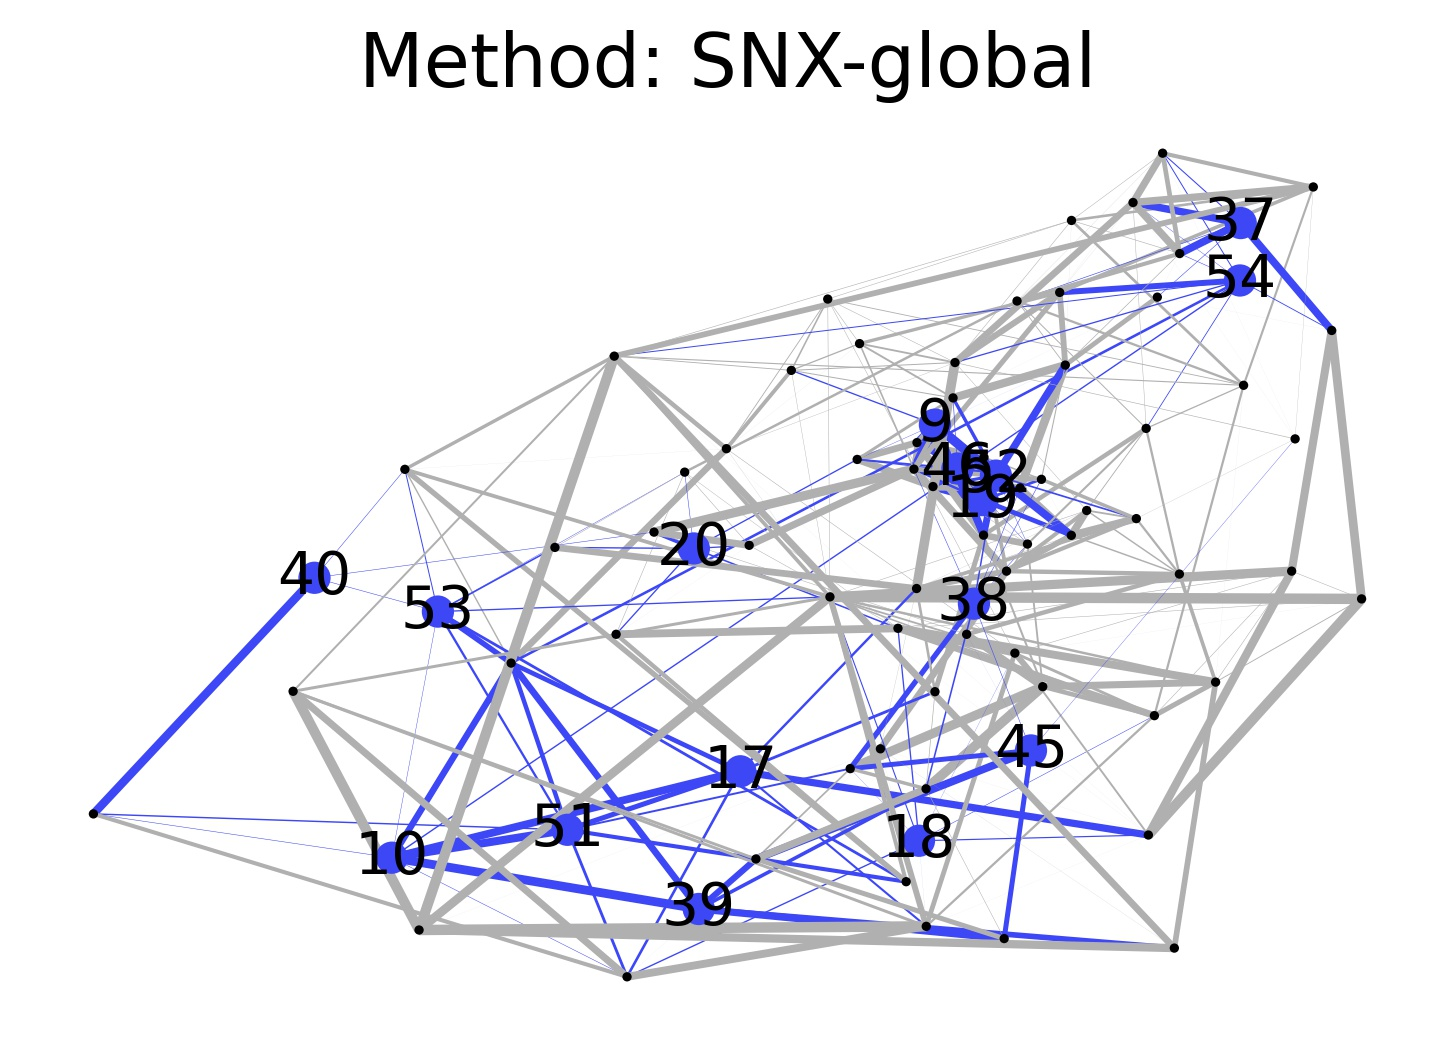}
\end{minipage}%
\begin{minipage}{.2\textwidth}
    \includegraphics[width=\textwidth]{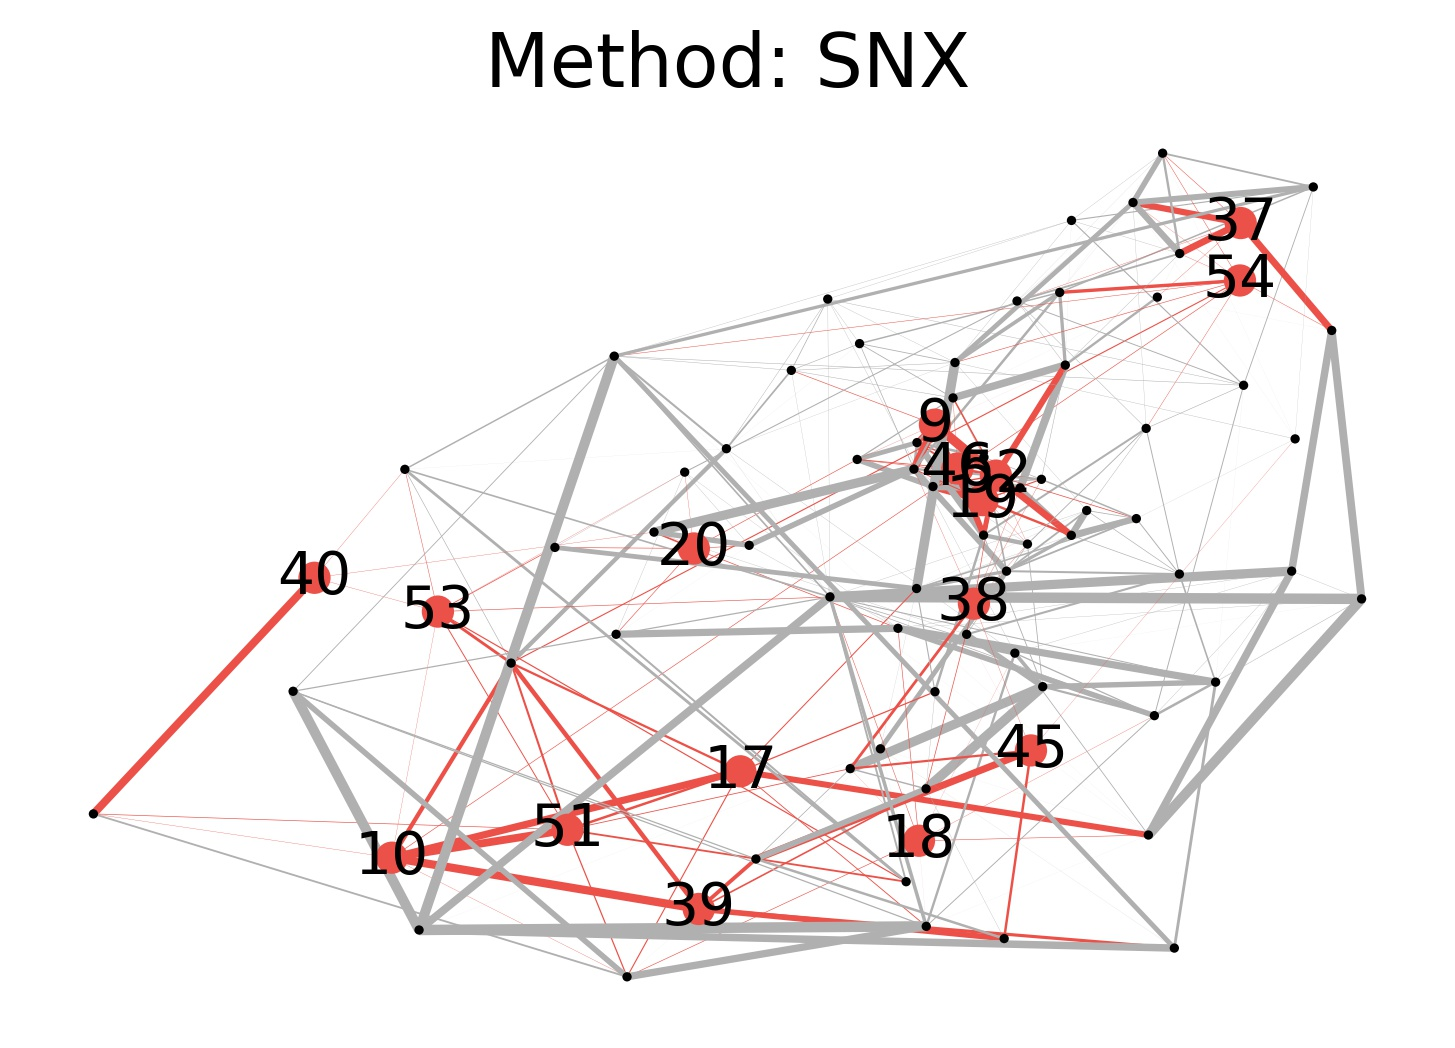}
\end{minipage}%
\begin{minipage}{.2\textwidth}
    \includegraphics[width=\textwidth]{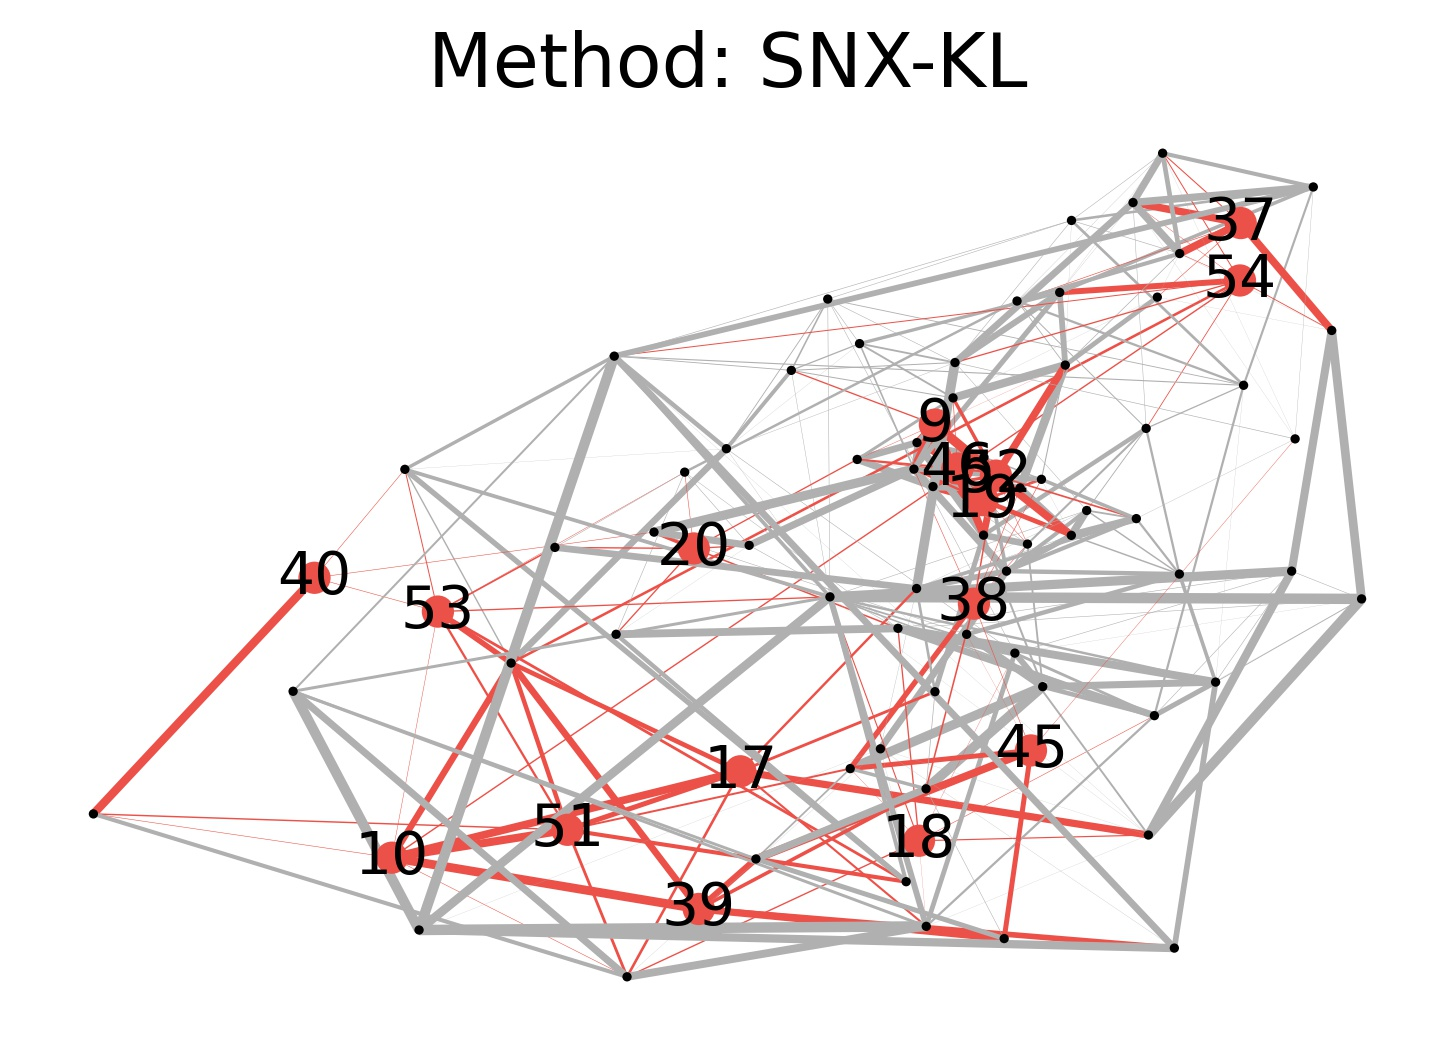}
\end{minipage}%
\begin{minipage}{.2\textwidth}
    \includegraphics[width=\textwidth]{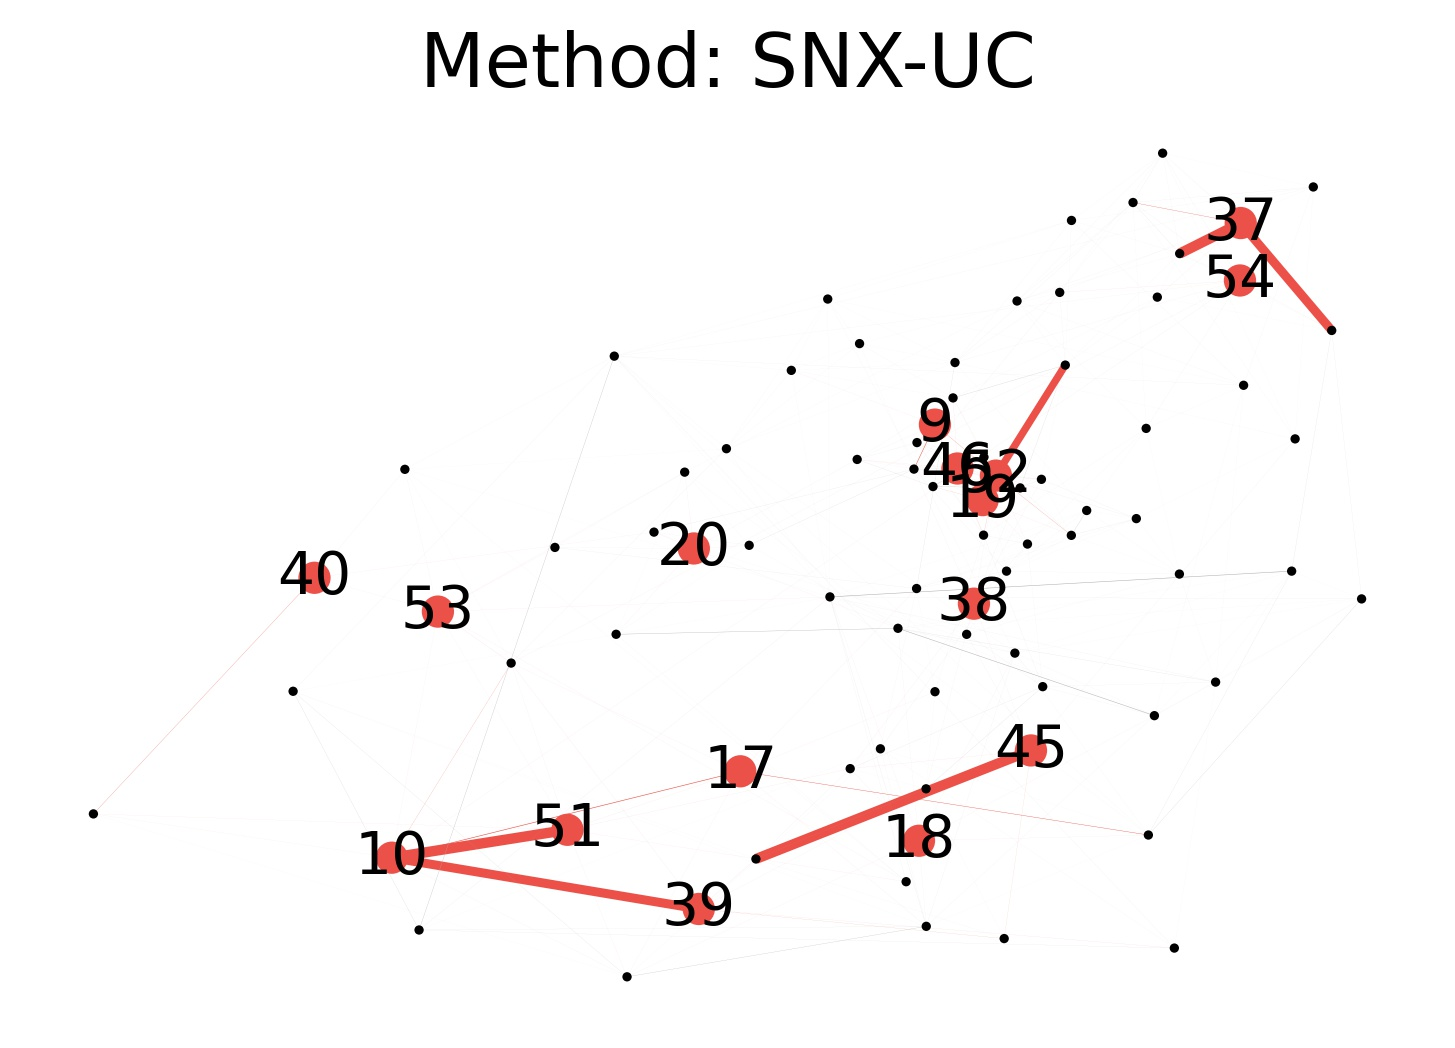}
\end{minipage}%
\begin{minipage}{.2\textwidth}
    \includegraphics[width=\textwidth]{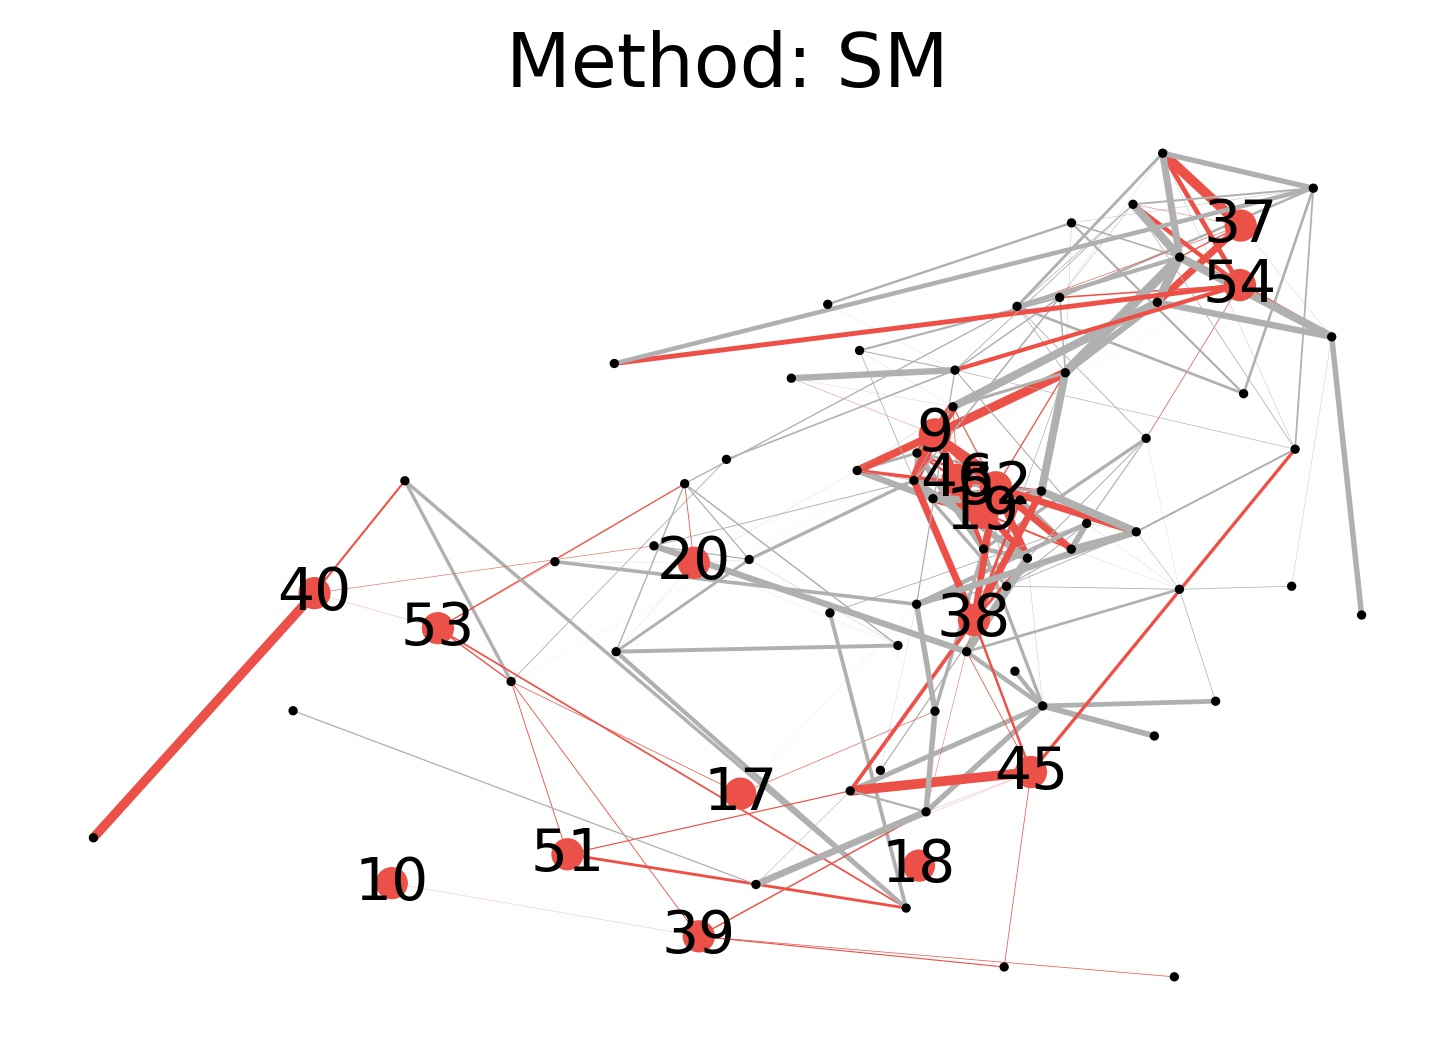}
\end{minipage}\\
    \caption{\small A case study for brain network in BP dataset.
    Blue highlights global edges selected by global masks and red highlights those by local masks.
    The large colored nodes represent the brain regions of the dorsal and ventral systems in human brain, which are shown highly correlated with Bipolar disorder by neuroscience studies. The thickness of edges indicates the importance of edges learned by the algorithm. 
    }
    \label{fig:bp_case_study_supp}
\end{figure*}

Figure \ref{fig:global_faithfulness} displays the sensitivity of the \textit{global} masks' performance found by SNX-global and DES with respect to the number/percentage of selected features on tabular datasets and edges on graph datasets.
It shows more and comprehensive results than Figure \ref{fig:sensitivity}.
Similar to the conclusions in Section \ref{sec:sensitivity_analysis},
on tabular data, 
the global masks generated can preserve good performance even selecting limited (less than 10) features,
and reach the best performance when the number of picked features is the same as the number of major features.
% on graph datasets,
% A higher percentage of edges is needed to retain the connection patterns on the Molecule dataset.
On the BP dataset, only about 20\% of the most important edges are needed to preserve the target SN's predictions closely.

Figure \ref{fig:local_faithfulness} evaluates the sensitivity of the performance of the \textit{local} masks
supplementing Figure \ref{fig:sensitivity}.
On tabular datasets, 
local masks achieve near-best faithfulness with much fewer picked features.
Moreover, the near-best counterfactual requires more selected features.
On Molecule, it requires less edge to obtain better faithfulness in the local masks than in the global masks, 
since stage 2 optimization can customize the global masks to accommodate specific references.
The two metrics of the local masks on the BP dataset behave similarly to the global masks.

% \begin{figure}
%     \centering
%     \includegraphics[width=0.45\textwidth]{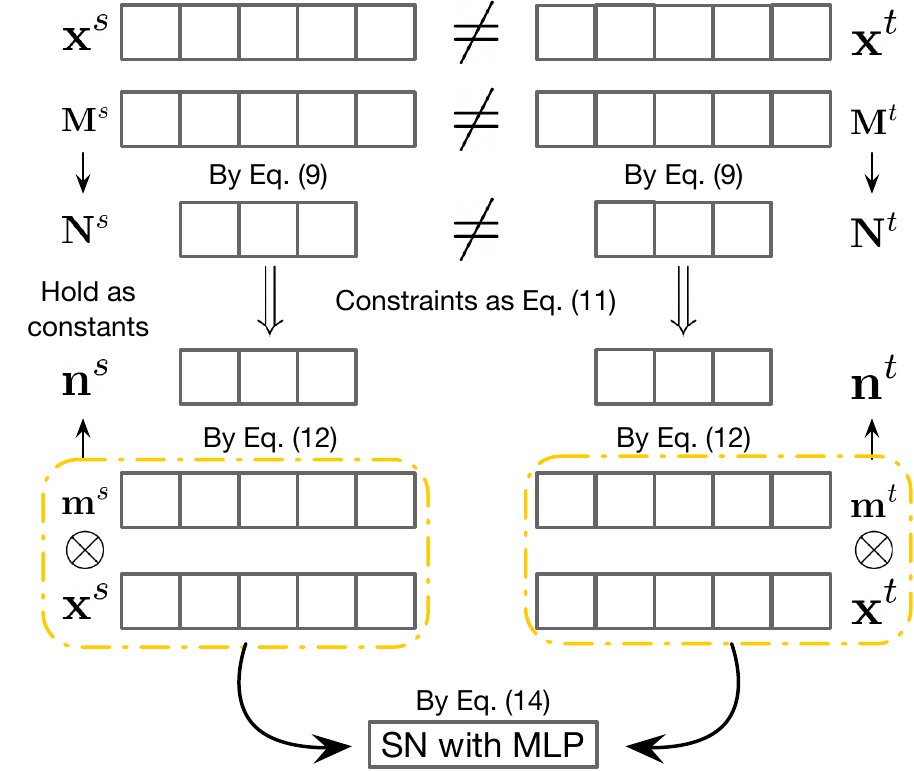}
%     \caption{
%     \footnotesize
%     Notations and relations among these notations in TABULAR data.
%     }
%     \label{fig:notation-tab}
% \end{figure}

% \begin{figure}
%     \centering
%     \includegraphics[width=0.45\textwidth]{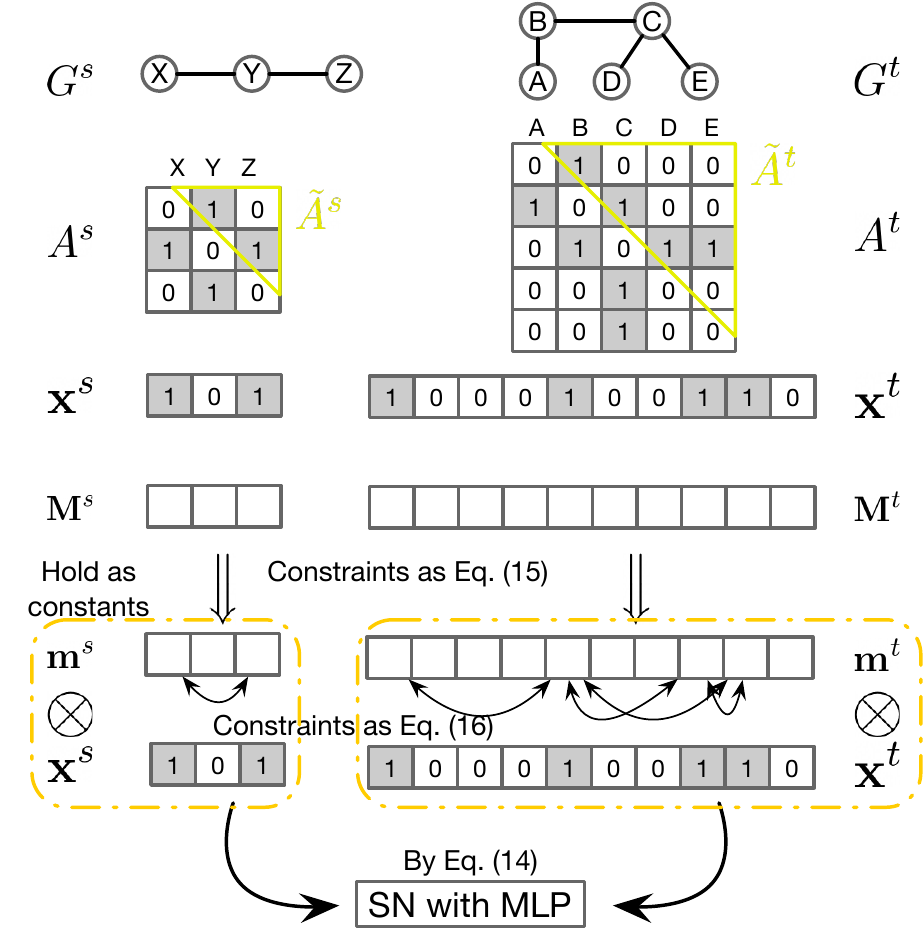}
%     \caption{
%     \footnotesize
%     Notations and relations among these notations in GRAPH data.
%     }
%     \label{fig:notation-graph}
% \end{figure}

\subsection{More on conformity}

% \begin{figure}[t]
%     \centering
% \begin{minipage}{.15\textwidth}
%     \includegraphics[width=\textwidth]{figs/adult_compare_kl_lag_break.jpg}
% \end{minipage}%
% \begin{minipage}{.15\textwidth}
%     \includegraphics[width=\textwidth]{figs/bank_compare_kl_lag_break.jpg}
% \end{minipage}%
% \begin{minipage}{.15\textwidth}
%     \includegraphics[width=\textwidth]{figs/credit_compare_kl_lag_break.jpg}
% \end{minipage}\\
% \begin{minipage}{.15\textwidth}
%     \includegraphics[width=\textwidth]{figs/compas_compare_kl_lag_break.jpg}
% \end{minipage}%
% \begin{minipage}{.15\textwidth}
%     \includegraphics[width=\textwidth]{figs/molecule_break_constraints.jpg}
% \end{minipage}%
% \begin{minipage}{.15\textwidth}
%     \includegraphics[width=\textwidth]{figs/BP_fmri_break_constraints.jpg}
% \end{minipage}
%     \caption{\small Comparing the ratio of instances breaking constraints in the first 200 iterations (in four tabular datasets) and 400 iterations (in two graph datasets) by using SNX-KL and SNX.
%     % \textcolor{blue}{Settings: We record the intermediate local masks (float-type) and compare it with the fixed global masks (float-type), to see the ratio of violations during optimizations.
%     % 'Ratio' here means: # of violations / # of constraints.}
%     }
%     \label{fig:kl-lag}
% \end{figure}

Fig. \ref{fig:kl-lag} 
% in the supplement further 
compares the violation of constraints by SNX and SNX-KL during optimization iterations in all six datasets.
To make both methods comparable,
we set hyper-parameters as the same:
In tabular data, 
we use learning rate $\eta_1 =10^{-1}, \eta_2=10^{-3}$;
and in graph data,
we set learning rate $\eta_1 = \eta_2=10^{-4}$;
besides,
we set the number of iterations for pretraining as 0 to ensure SNX-KL and SNX to start from the same initialization.
SNX breaks less constraints in four tabular datasets.
SNX-KL follows more in the Molecule. 
As for BP,
SNX-KL keeps violating about 30\% of constraints after about 70 iterations.
We conjecture the reason is that SNX-KL converges to a ``minimizer'' balancing both objective functions and soft constraints.

\subsection{Convergence of GDA}

Figure \ref{fig:grads_complete} shows the trends of the norm of $\mathbf{m}$ and $\boldsymbol{\lambda}$ when running GDA on all six datasets,
which provides more comprehensive results for evaluating the convergence of GDA in Section \ref{sec:convergence}.

\subsection{Case studies}
\noindent\textbf{Adult Dataset}.
Figure \ref{tab:case_study} is based on the same data and coloring schema in Table~\ref{tab:simplified_case_study} but provides values of the query and rerence instances
% a comprehensive case study 
from the Adult dataset.
% The coloring schema is the same as in Table~\ref{tab:simplified_case_study}.
% As mentioned in Section \ref{sec:quali},
% the query's features are shown in the center of the table, 
% and the salient global features are colored blue.
% The two references' features are above and below the query's,
% whose salient local features found by the three methods (SM, SNX-UC, and SNX) are colored red.
% The color saturation levels indicate the importance of the features.
% For example, 
% the query's \texttt{Workclass, Education, Hours/week} and \texttt{Occupation} are highlighted by dark blue by SNX-global,
% which means these features are considered key factors resulting in the ``Below 50k'' prediction.
% Global masks either come from self-supervised learning or domain knowledge.
% In other words,
% self-supervised learning shows that \texttt{Age}, for example, cannot significantly contribute to the prediction of someone's income.
% or it is possible that domain knowledge fixes \texttt{Age} for the sake of fairness.
% Both cases call for the obedience of the local masks.
% Considering the local masks highlighted in red in the two references,
% we notice that
% the color saturation level of each entry in SNX is the same or lighter than the corresponding one in SNX-global, 
% indicating SNX follows the global constraints set by SNX-global.
% However,
% SM and SNX-UC highlight some features that are lightly colored by SNX-global,
% such as \texttt{Age, Race} and \texttt{Sex}.
Specifically,
the feature \texttt{Age} highlighted by SM is indeed one of the different features between the query and the second reference,
while it violates the global constraint of ``not selecting \texttt{Age}'', set by SNX-global.

\vspace{.1in}
\noindent\textbf{BP Dataset}.
Figure~\ref{fig:bp_case_study_supp} shows some masks learned on the BP dataset.
The first graph represents the global mask found by SNX-global,
and the remaining four graphs are local masks found by four methods.
The larger colored nodes are brain regions of interest (ROIs) related to the human dorsal and ventral systems, such as ventromedial prefrontal cortex (node \#39), anterior cingulate cortex, the dorsolateral prefrontal cortex (\#17), the superior parietal lobule (\#10), and the anterior cingulate cortex (\#51), which relates to emotion processing, emotion regulation and reward processing. These regions and the associated functions could be highly affected by the bipolar disorder according to neuroscience studies \cite{chen2011quantitative,zovetti2020default}. 
The edges connected to these nodes are colored accordingly. 

In the figure,
many edges adjoined to these ROIs are captured by the global invariant mask.
In particular, the interconnections among the aforementioned four ROIs (\#39, \#17, \#10 and \#51) are well captured by SNX-global.
This indicates that SNX-global can generate interpretable and meaningful masks for neurological analysis.

In Figure~\ref{fig:bp_case_study}, the thickness of edges indicates the importance of edges in different masks.
It is clear that both SNX and SNX-KL found local masks conformal to the constraints set by the global mask in the first graph.
% shown by the thickness of edges being the same or thinner than SNX-global's.
SNX-UC highlights only few edges and assign near-zeros to the remaining edges (the almost invisible ones).
% This is because SNX-UC optimizes Eq. (\ref{eq:con_lm_obj}),
% and
% the faithfulness loss function $\ell$ drives it to pick salient edges while
% the $\ell-1$ regularization forces it to give up most of edges.
% SM may select some trivial edges by SNX-global.

\subsection{Datasets Statistics and model details}
\noindent \textbf{Datasets Statistics.}
Table \ref{tab:datasets} shows the datasets' details for experiments, 
including four tabular datasets and two graph datasets.
\textit{Adult} \cite{mothilal2020explaining} is used to predict if a person's annual income would be over 50 thousand dollars or not.
\textit{Bank} \cite{moro2014data} is used to predict if a person will subscribe to a term deposit.
\textit{Credit} \cite{mothilal2020explaining} is used for evaluating a person's credit risks.
\textit{COMPAS} \cite{mothilal2020explaining} is used for tracking and predicting the reoffending of criminal defendants.
\textit{Molecule} \cite{Duvenaud2015,jin2018junction} is used to predict if a molecule is a protein or not.
\textit{BP} \cite{ma2019deep} is used to predict if a potential patient has bipolar or healthy by evaluating the connection patterns in the subjects' brain networks.

\begin{table}[h]
    % \centering
    \scriptsize
    % \footnotesize
    % \captionsetup{font=footnotesize}
    \caption{ \small Datasets statistics 
    % \textcolor{red}{may be moved to the appendix}
    }
    \subcaption*{Tabular data statistics}
    \begin{tabular}{c|c|c|c|c}
    \toprule
    Dataset & \# instances & \# major features & \# minor features & \# explain pairs \\
    \midrule
    Adult & 45222 & 9 & 28 & 20000 \\
    Bank & 30488 & 8 & 18 & 20000\\
    Credit & 1000 & 9 & 27 & 18000\\
    COMPAS & 6172 & 6 & 16 & 20000\\
    \bottomrule
    \end{tabular}
    \scriptsize
    \subcaption*{Graph data statistics}
    \begin{tabular}{c|c|c|c|c|c}
    \toprule
    Dataset & \# graphs & \# nodes & \# edges & \# features & \# explain pairs\\
    \midrule
    Molecule & 200 & 10.77 & 9.77 & 1068 & 320\\
    BP & 90 & 82 & 315.84 & 82 & 216\\
    \bottomrule
    \end{tabular}
    \label{tab:datasets}
\end{table}

\noindent \textbf{Siamese network architectures.}
To achieve the best accuracy performance, 
we try different structures including number of layers and the embedding dimensions in each layer.
For all tabular datasets,
the target SN model is an MLP with a single hidden layer of dimension 16 as the mapping function $emb(\mathbf{x}; \boldsymbol{\theta})$,
% = \theta_1^\top\mathbf{x}$ + $\theta_0$,
cosine similarity as the similarity function,
The SN is trained using the hinge loss
$\ell^{SN} = \textnormal{max}\{0, 1-y_{st} * f(\mathbf{x}^s, \mathbf{x}^t; \boldsymbol{\theta}) \}$.

For graph data,
the target SN is a two-layer GCN (with dimensions 256 and 128, respectively) following a mean pooling layer as the mapping function,
the euclidean distance as graph similarity metrics,
The SN is trained using the loss $\ell^{SN} = y_{st} * [f(\mathbf{x}^s, \mathbf{x}^t; \boldsymbol{\theta})]^2 + 
(1-y_{st}) [ \max \{0, \textnormal{margin} - f(\mathbf{x}^s, \mathbf{x}^t; \boldsymbol{\theta}) \} ]^2 $ (margin=4).

\noindent \textbf{Hyperparameters of SNX.}
On the tabular datasets,
to extract global masks,
learning rate is $10^{-1}$, and $MaxIter=50$,
$\gamma=10^{-3}$ in Eq. (\ref{eq:obj_gm}) 
and $\gamma=10^{-3}$ in Eq. (\ref{eq:con_lm_obj}).
To extract local masks,
$\eta_1=10^{-1},\eta_2=10^{-3}$ in Eq. (\ref{eq:variable_update}),
and 
% pretrain for 50 iterations and 
$PreIter=50, MaxIter=100$.
% $\gamma=10^{-3}$ in Eq. (\ref{eq:con_lm_tabular_obj}).

To extract global masks on graph datasets,
learning rate is $10^{-1}$, and $MaxIter=200$,
$\gamma$ in Eq. (\ref{eq:obj_gm}) and Eq. (\ref{eq:con_lm_obj}) is $10^{-1}$ for Molecule and $10^{-4}$ for BP.
To extract local masks,
$ \eta_1=10^{-1}, \eta_2=10^{-3}$ in Eq. (\ref{eq:variable_update}).
There is no pretrain epoch and $MaxIter=400$.

For all experiments, $\beta$ in SNX-KL is set as 1.

\noindent{}\textbf{Experimental environments and running time.}
\begin{itemize}[leftmargin=*,noitemsep,topsep=0pt]
    \item Hardware: 
    we conduct most of the experiments on a Macbook Pro with an six-core i9 Intel CPU and 32G memory. 
    \item Software:
    we run with Python (3.8.1), Numpy (1.18.5), Pytorch(1.6.0), and all random seeds are set as 24.
    \item Running time:
    % Training the target models can be finished in 5 minutes in all datasets.
    % As for generating 
    To generate masks for explanations,
    each variant of SNX, such as SNX, SNX-UC, SNX-KL,
    takes about 1 hour for all explaining pairs in tabular data
    % which is about 0.18 seconds per pair,
    (0.18 s/pair),
    about 30 minutes in Molecule
    % which is about 5.5 seconds per pair,
    (5.5 s/pair),
    and about 12 hours in BP
    % which is about 3 minutes per pair.
    (3 mins/pair).
\end{itemize}
